# Supplementary material for: Projective Spacetime Symmetry of Spacetime Crystals
Source: arXiv:2310.09577 source file (2023-10-14)
Supplement: Supplementary file 1 [file supp.pdf]

# Supplemental information for
# "Projective Spacetime Symmetry of Spacetime Crystals"

Zheng Zhang,[1,2] Z. Y. Chen,[1,2] and Y. X. Zhao[3,4,*]

[1]*National Laboratory of Solid State Microstructures and Department of Physics, Nanjing University, Nanjing 210093, China*
[2]*The University of HongKong Shenzhen Institute of Research and Innovation, Shenzhen 518057, China*
[3]*Department of Physics and HKU-UCAS Joint Institute for Theoretical and Computational Physics at Hong Kong, The University of Hong Kong, Pokfulam Road, Hong Kong, China*
[4]*HK Institute of Quantum Science & Technology, The University of Hong Kong, Pokfulam Road, Hong Kong, China*

## Contents

**A. Background** 2
1. Projective representation and multiplier 2
2. Projective symmetry algebra and cohomology invariants 3

**B. Projective symmetry algebras of (1,1)D spacetime crystalline groups** 4
1. P1 5
2. P2 6
3. $\mathrm{Pm_x}$ 7
4. $\mathrm{Pm_t}$ 8
5. $\mathrm{Pm_xm_t}$ 9
6. $\mathrm{Pg_x}$ 10
7. $\mathrm{Pg_t}$ 10
8. $\mathrm{Pg_xg_t}$ 11
9. $\mathrm{Pm_xg_t}$ 12
10. $\mathrm{Pm_tg_x}$ 13
11. $\mathrm{Cm_x}$ 14
12. $\mathrm{Cm_t}$ 14
13. $\mathrm{Cm_xm_t}$ 15

**C. Time crystals with gauge structures** 16
1. Electric A-B effect and electric flux 16
2. Symmetries of spacetime tight binding models with gauge structures 17
3. Flux interpretation of cohomology invariants 18
   i. Cohomology invariants of translation subgroups 18
   ii. Cohomology invariants of rotations 19
   iii. Cohomology invariants between translations and reflections 20
   iv. Cohomology invariants between translations and glide-reflections 20
   v. Cohomology invariants of reflections 21

**D. Lattice realization of projective symmetry algebras of (1,1)D spacetime crystalline groups** 22
1. P1 22
2. P2 23
3. $\mathrm{Pm_x}$ 23
4. $\mathrm{Pm_t}$ 24
5. $\mathrm{Pm_xm_t}$ 25
6. $\mathrm{Pg_x}$ 25
7. $\mathrm{Pg_t}$ 26

*yuxinphy@hku.hk

8. $\mathrm{Pg_xg_t}$ 26
9. $\mathrm{Pm_xg_t}$ 27
10. $\mathrm{Pm_tg_x}$ 27
11. $\mathrm{Cm_x}$ 28
12. $\mathrm{Cm_t}$ 29
13. $\mathrm{Cm_xm_t}$ 29

**E. Other details** 30
1. Proof of the electric Floquet-Bloch theorem 30
2. Kramers degeneracy protected by projective P2 symmetry 31
3. Band crossing due to projective symmetry 32
4. Parameters of models 33

**F. References** 36

## A. Background

### 1. Projective representation and multiplier

An $\mathcal{A}$-projective representation of group $G$ is a vector space $V$, with a map $\rho : G \to GL(V)$ which is "almost a homomorphism" in the sense that

$$\rho(g_1)\rho(g_2) = \nu(g_1, g_2)\rho(g_1 g_2), \quad \forall g_1, g_2 \in G, \tag{1}$$

where function $\nu : G \times G \to \mathcal{A}$ is called a multiplier for $G$.

Associativity $(g_1 g_2)g_3 = g_1(g_2 g_3)$ requires the multiplier $\nu$ satisfy the 2-cocycle equation:

$$\nu(g_1, g_2)\nu(g_1 g_2, g_3) = \nu(g_2, g_3)\nu(g_1, g_2 g_3), \quad \forall g_1, g_2, g_3 \in G. \tag{2}$$

We denote the set of all 2-cocycles by $Z^2(G, \mathcal{A})$, which is an abelian group under the multiplication of functions. Two projective representations $\rho$ and $\rho'$ related by $\rho'(g) = \chi(g)\rho(g)$ are considered as equivalent, where $\chi(g) \in \mathcal{A}$. Correspondingly, their multipliers $\nu, \nu'$ is related by

$$\nu'(g_1, g_2) = \nu(g_1, g_2)\frac{\chi(g_1)\chi(g_2)}{\chi(g_1 g_2)}. \tag{3}$$

A function $f : G \times G \to \mathcal{A}$ in the form $f(g_1, g_2) = \chi(g_1)\chi(g_2)/\chi(g_1 g_2)$ or $f(g_1, g_2) = \chi(g_1 g_2)/\chi(g_1)\chi(g_2)$ is called a 2-coboundary. Two 2-cocycles is equivalent if they differ by a 2-coboundary. We denote the set of all 2-coboudaries by $B^2(G, \mathcal{A})$, which is also an abelian group under the multiplication of functions. Then, the set of nonequivalent multipliers (2-cocycles) is given by the quotient group

$$H^2(G, \mathcal{A}) = Z^2(G, \mathcal{A})/B^2(G, \mathcal{A}), \tag{4}$$

which is called the second cohomology group. Thus, $H^2(G, \mathcal{A})$ classifies nonequivalent $\mathcal{A}$-valued multipliers for $G$.

In quantum mechanics, time-reversal operations are represented by anit-unitary operators rather than unitary operators. Therefore they have complex conjugate action on the $\mathcal{A}$-valued multiplier $\nu$ (in general $\mathcal{A} = U(1)$). Consequently, if $G$ contains time-reversal elements, the 2-cocycle equation should be modified to a twisted 2-cocycle equation:

$$\nu(g_1, g_2)\nu(g_1 g_2, g_3) = \widetilde{g_1}(\nu(g_2, g_3))\nu(g_1, g_2 g_3), \quad \forall g_1, g_2, g_3 \in G, \tag{5}$$

where $\widetilde{g}$ is complex conjugate if $\rho(g)$ is anti-unitary, otherwise $\widetilde{g}$ is trivial. We denote the set of twisted 2-cocycles as $Z^{2,c}(G, \mathcal{A})$, where $c$ indicate the complex conjugate action. In a similar manner, the 2-coboundaries now should also be twisted, taking the form $\chi(g_1)\widetilde{g_1}(\chi(g_2))/\chi(g_1 g_2)$ or $\chi(g_1 g_2)/\chi(g_1)\widetilde{g_1}(\chi(g_2))$. We denote the set of them by $B^{2,c}(G, \mathcal{A})$. The nonequivalent multipliers are now classfied by the twisted second cohomology group

$$H^{2,c}(G, \mathcal{A}) = Z^{2,c}(G, \mathcal{A})/B^{2,c}(G, \mathcal{A}). \tag{6}$$

## 2. Projective symmetry algebra and cohomology invariants

The multiplicative relations of a projective representations is called a *projective symmetry algebra*. It is determined by the multiplicative relations of group elements and the multiplier $\nu$. However, the multiplier is typically complicated and contains much redundancy. To concisely capture the essential information of the projective symmetry algebra, we use projective symmetry algebraic relations of generators and *cohomology invariants*, which will be introduced below.

A finite generated group $G$ can be presented by generators and relations:

$$G = \langle \mathcal{S} | \mathcal{R} \rangle, \tag{7}$$

where $\mathcal{S} = \{s_1, s_2, ...\}$ is the set of generators and $\mathcal{R} = \{r_1(s), r_2(s), ...\}$ is the set of relations. In general, the relations have the following form :

$$r_i(s) = s_{i_1}^{n_1} \cdot s_{i_2}^{n_2} \cdot ... \cdot s_{i_f}^{n_f} = 1. \tag{8}$$

Two "words" $w = s_1^{n_1} s_2^{n_2}...$ and $w' = s_1^{n_1'} s_2^{n_2'}...$ correspond to the same group element if they can be reduced to be equal using relations.

If $\rho$ is a representation of $G$, its constrain on generators also satisfies the algebraic relations in $\mathcal{R}$, because

$$r_i(\rho(s)) = \rho(s_{i_1})^{n_1} \rho(s_{i_2})^{n_2} ... \rho(s_{i_f})^{n_f} = \rho(s_{i_1}^{n_1} \cdot s_{i_2}^{n_2} \cdot ... \cdot s_{i_f}^{n_f}) = 1. \tag{9}$$

However, if $\rho$ is a projective representation of $G$ with multiplier $\nu$, its constrain on generators does not satisfy the algebraic relations in $\mathcal{R}$, but with additional phases, for example,

$$r_i(\rho(s)) = \rho(s_{i_1})^{n_1} \rho(s_{i_2})^{n_2} ... \rho(s_{i_f})^{n_f} = \alpha_i \rho(s_{i_1}^{n_1} \cdot s_{i_2}^{n_2} \cdot ... \cdot s_{i_f}^{n_f}) = \alpha_i. \tag{10}$$

The occurance of $\alpha_i$ is due to the multiplier $\nu$ of the projective representation. If we define a "modified" presentation $\widetilde{G} = \langle \mathcal{S} | \widetilde{\mathcal{R}} \rangle$, where $\widetilde{\mathcal{R}} = \{r_1(s) = \alpha_1, r_2(s) = \alpha_2, ...\}$ is the projective symmetry algebraic relations of generators. Then the constrain of $\rho$ on $\mathcal{S}$ satisfies the relations in $\widetilde{\mathcal{R}}$. In the "modified" presentation, two words correspond to the same group element if they can be reduced to be equal up to a phase using relations.

Now, we state the core conclusion of this section: The "modified" presentation $\widetilde{G} = \langle \mathcal{S} | \widetilde{\mathcal{R}} \rangle$ contains the information of the equivalence class of multiplier $\nu$. More concretly, if $\widetilde{G}$ is obtained by modifying $\mathcal{R}$ to $\widetilde{\mathcal{R}}$ due to multiplier $\nu$, we can infer the equivalence class of multiplier $\nu$ from $\widetilde{G}$, though $\nu$ itself cannot be inferred. This conclusion is very useful because it tells us that to capture the information of a projective symmetry algebra (in an equivalent sense), we only need a "modified" presentation $\widetilde{G} = \langle \mathcal{S} | \widetilde{\mathcal{R}} \rangle$, which is much simpler than the multiplier.

To prove this conclusion, we proceed as follows. For a fixed $\mathcal{S}$, we can assign a "standard" word $w(g) = s_1^{n_1} s_2^{n_2} s_3^{n_3} \dots$ to each group element $g \in G$. Then for a given $\widetilde{G} = \langle \mathcal{S} | \widetilde{\mathcal{R}} \rangle$, we can obtain a multiplier $\widetilde{\nu}$ by

$$w(g_a)w(g_b) = s_1^{n_{a_1}} s_2^{n_{a_2}} s_3^{n_{a_3}} ... s_1^{n_{b_1}} s_2^{n_{b_2}} s_3^{n_{b_3}} ... = \widetilde{\nu}(g_a, g_b) s_1^{n_{c_1}} s_2^{n_{c_2}} s_3^{n_{c_3}} ... = \widetilde{\nu}(g_a, g_b) w(g_c), \tag{11}$$

where $g_c = g_a g_b$ and the multiplier $\widetilde{\nu}$ is obtained by using the relations in $\widetilde{\mathcal{R}}$. We now prove $\widetilde{\nu}$ is in the equivalence class of $\nu$. From $\rho(g_a)\rho(g_b) = \nu(g_a, g_b)\rho(g_c)$, we have

$$\begin{aligned} \rho(s_1^{n_{a_1}} s_2^{n_{a_2}} s_3^{n_{a_3}} ...)\rho(s_1^{n_{b_1}} s_2^{n_{b_2}} s_3^{n_{b_3}} ...) &= \nu(g_a, g_b)\rho(s_1^{n_{c_1}} s_2^{n_{c_2}} s_3^{n_{c_3}} ...) \\ \chi(g_a)\widetilde{g_a}(\chi(g_b))\rho(s_1^{n_{a_1}})\rho(s_2^{n_{a_2}})\rho(s_3^{n_{a_3}})...\rho(s_1^{n_{b_1}})\rho(s_2^{n_{b_2}})\rho(s_3^{n_{b_3}})... &= \nu(g_a, g_b)\chi(g_c)\rho(s_1^{n_{c_1}})\rho(s_2^{n_{c_2}})\rho(s_3^{n_{c_3}})... \\ \chi(g_a)\widetilde{g_a}(\chi(g_b))\widetilde{\nu}(g_a, g_b)\rho(s_1^{n_{c_1}})\rho(s_2^{n_{c_2}})\rho(s_3^{n_{c_3}})... &= \nu(g_a, g_b)\chi(g_c)\rho(s_1^{n_{c_1}})\rho(s_2^{n_{c_2}})\rho(s_3^{n_{c_3}})... \\ \frac{\chi(g_a)\widetilde{g_a}(\chi(g_b))}{\chi(g_a g_b)}\widetilde{\nu}(g_a, g_b) &= \nu(g_a, g_b), \end{aligned} \tag{12}$$

where $\chi(g_i)$ is the phase due to decomposing $\rho(s_1^{n_{i_1}} s_2^{n_{i_2}} s_3^{n_{i_3}} ...) = \chi(g_i)\rho(s_1^{n_{i_1}})\rho(s_2^{n_{i_2}})\rho(s_3^{n_{i_3}})...$. Thus we complete the proof.

Although the "modified" presentation is more concise than the multiplier, it may still contain redundancies. Let us consider a "modified" presentation $\widetilde{G} = \langle s_1, s_2, ... | r_1(s) = \alpha_1, r_2(s) = \alpha_2, ... \rangle$. For each generator $s$, we can do a coboundary transformation $s \to s' = \chi(s)s$, which changes the relations $\widetilde{\mathcal{R}}$ to $\widetilde{\mathcal{R}'} = \{r_1(s') = \alpha_1', r_2(s') = \alpha_2' ...\}$. This yields a new "modified" presentation $\langle s_1, s_2, ... | r_1(s) = \alpha_1', r_2(s) = \alpha_2', ... \rangle$, which corresponds to the same cohomology class of multipliers as $\widetilde{G}$. To reduce this redundancy, we can recombine the relations such that some factors are invariant under coboundary transformations while others can be set to 1. We call a factor that is invariant under coboundary transformations a cohomology invariant. The values of a complete set of cohomology invariants uniquely determine the equivalence class of a multiplier (and hence the projective symmetry algebra).

In the following sections, we will utilize "modified" presentation and cohomology invariants to describe projective symmetry algebras.

### B. Projective symmetry algebras of (1,1)D spacetime crystalline groups

In this section, we derive all the nonequivalent $U(1)$ and $\mathbb{Z}_2$ projective symmetry algebras for all 13 (1,1)D spacetime crystalline groups. The results are summarized in Table. I and Table. II.

| $G_{st}$ | $H^{2,c}_{U(1)}$ | Generators | Cohomology invariants | N |
|---|---|---|---|---|
| $P1$ | $U(1)$ | $L_1, L_2$ | $[\mathsf{L}_1 : \mathsf{L}_2] = \sigma$ | $U(1)$ |
| $P2$ | $\mathbb{Z}_2^4$ | $L_1, L_2, C$ | $\mathsf{C}^2 = \alpha_1,\ (\mathsf{L}_1\mathsf{C})^2 = \alpha_2,\ (\mathsf{L}_2\mathsf{C})^2 = \alpha_3,\ (\mathsf{L}_1\mathsf{L}_2\mathsf{C})^2 = \alpha_4$ | 7 |
| $Pm_x$ | $\mathbb{Z}_2^2$ | $L_x, L_T, M_x$ | $[\mathsf{M}_x : \mathsf{L}_T] = \eta_1,\ [\mathsf{L}_x\mathsf{M}_x : \mathsf{L}_T] = \eta_2,\ \mathsf{M}_x^2 = 1,\ (\mathsf{L}_x\mathsf{M}_x)^2 = 1$ | 3 |
| $Pm_t$ | $U(1)\times\mathbb{Z}_2^2$ | $L_x, L_T, M_t$ | $[\mathsf{L}_x : \mathsf{L}_T] = \sigma,\ [\mathsf{M}_t : \mathsf{L}_x] = 1,\ \mathsf{M}_t^2 = \beta_1,\ (\mathsf{L}_T\mathsf{M}_t)^2 = \beta_2$ | $U(1)\times 3$ |
| $Pm_xm_t$ | $\mathbb{Z}_2^6$ | $L_x, L_T, M_x, M_t$ | $(\mathsf{M}_x\mathsf{M}_t)^2 = \alpha_1,\ (\mathsf{L}_x\mathsf{M}_x\mathsf{M}_t)^2 = \alpha_2,\ (\mathsf{L}_T\mathsf{M}_x\mathsf{M}_t)^2 = \alpha_3,\ (\mathsf{L}_x\mathsf{L}_T\mathsf{M}_x\mathsf{M}_t)^2 = \alpha_4,$ $\mathsf{M}_x^2 = 1,\ (\mathsf{L}_x\mathsf{M}_x)^2 = 1,\ \mathsf{M}_t^2 = \beta_1,\ (\mathsf{L}_T\mathsf{M}_t)^2 = \beta_2$ | 24 |
| $Pg_x$ | 1 | $L_x, g_x$ | $\mathsf{g}_x\mathsf{L}_x\mathsf{g}_x^{-1}\mathsf{L}_x = 1$ | 1 |
| $Pg_t$ | $U(1)$ | $L_T, g_t$ | $\mathsf{g}_t\mathsf{L}_T\mathsf{g}_t^{-1}\mathsf{L}_T = \tau$ | $U(1)$ |
| $Pg_xg_t$ | $\mathbb{Z}_2^2$ | $g_x, g_t$ | $(\mathsf{g}_x\mathsf{g}_t)^2 = \alpha_1,\ (\mathsf{g}_x\mathsf{g}_t^{-1})^2 = \alpha_2$ | 3 |
| $Pm_xg_t$ | $\mathbb{Z}_2^3$ | $L_T, M_x, g_t$ | $[\mathsf{M}_x : \mathsf{L}_T] = \eta,\ (\mathsf{M}_x\mathsf{g}_t)^2 = \alpha_1,\ (\mathsf{L}_T\mathsf{M}_x\mathsf{g}_t)^2 = \alpha_2,\ \mathsf{M}_x^2 = 1$ | 6 |
| $Pm_tg_x$ | $\mathbb{Z}_2^3$ | $L_x, M_t, g_x$ | $[\mathsf{M}_t : \mathsf{L}_x] = 1,\ (\mathsf{M}_t\mathsf{g}_x)^2 = \alpha_1,\ (\mathsf{L}_x\mathsf{M}_t\mathsf{g}_x)^2 = \alpha_2,\ \mathsf{M}_t^2 = \beta$ | 6 |
| $Cm_x$ | $\mathbb{Z}_2$ | $L_1, L_2, M_x$ | $[\mathsf{L}_1 : \mathsf{L}_2] = \sigma,\ \mathsf{M}_x\mathsf{L}_1\mathsf{M}_x^{-1}\mathsf{L}_2^{-1} = 1,\ \mathsf{M}_x^2 = 1$ | 2 |
| $Cm_t$ | $U(1)\times\mathbb{Z}_2$ | $L_1, L_2, M_t$ | $[\mathsf{L}_1 : \mathsf{L}_2] = \sigma,\ \mathsf{M}_t\mathsf{L}_1\mathsf{M}_t^{-1}\mathsf{L}_2^{-1} = 1,\ \mathsf{M}_t^2 = \beta$ | $U(1)\times 2$ |
| $Cm_xm_t$ | $\mathbb{Z}_2^4$ | $L_1, M_x, M_t$ | $(\mathsf{M}_x\mathsf{M}_t)^2 = \alpha_1,\ (\mathsf{L}_1\mathsf{M}_x\mathsf{M}_t)^2 = \alpha_2,\ (\mathsf{L}_1\mathsf{M}_x\mathsf{L}_1^{-1}\mathsf{M}_t)^2 = \alpha_3,\ \mathsf{M}_x^2 = 1,\ \mathsf{M}_t^2 = \beta$ | 12 |

TABLE I: $U(1)$-projective symmetry algebras of 13 $(1,1)$D spacetime groups. Factors $\alpha, \beta, \eta$ are valued in $\mathbb{Z}_2 = \{\pm 1\}$, and factors $\tau, \sigma$ are valued in $U(1)$ except the $\sigma$ factor for $Cm_x$, which is valued in $\mathbb{Z}_2$.

| $G_{st}$ | $H^2_{\mathbb{Z}_2}$ | Generators | Cohomology invariants | N |
|---|---|---|---|---|
| $P1$ | $\mathbb{Z}_2$ | $L_1, L_2$ | $[\mathsf{L}_1 : \mathsf{L}_2] = \sigma$ | 2 |
| $P2$ | $\mathbb{Z}_2^4$ | $L_1, L_2, C$ | $\mathsf{C}^2 = \alpha_1,\ (\mathsf{L}_1\mathsf{C})^2 = \alpha_2,\ (\mathsf{L}_2\mathsf{C})^2 = \alpha_3,\ (\mathsf{L}_1\mathsf{L}_2\mathsf{C})^2 = \alpha_4$ | 7 |
| $Pm_x$ | $\mathbb{Z}_2^4$ | $L_x, L_T, M_x$ | $[\mathsf{M}_x : \mathsf{L}_T] = \eta_1,\ [\mathsf{L}_x\mathsf{M}_x : \mathsf{L}_T] = \eta_2,\ \mathsf{M}_x^2 = \gamma_1,\ (\mathsf{L}_x\mathsf{M}_x)^2 = \gamma_2$ | 10 |
| $Pm_t$ | $\mathbb{Z}_2^4$ | $L_x, L_T, M_t$ | $[\mathsf{M}_t : \mathsf{L}_x] = \overline{\eta}_1,\ [\mathsf{L}_T\mathsf{M}_t : \mathsf{L}_x] = \overline{\eta}_2,\ \mathsf{M}_t^2 = \beta_1,\ (\mathsf{L}_T\mathsf{M}_t)^2 = \beta_2$ | 10 |
| $Pm_xm_t$ | $\mathbb{Z}_2^8$ | $L_x, L_T, M_x, M_t$ | $(\mathsf{M}_x\mathsf{M}_t)^2 = \alpha_1,\ (\mathsf{L}_x\mathsf{M}_x\mathsf{M}_t)^2 = \alpha_2,\ (\mathsf{L}_T\mathsf{M}_x\mathsf{M}_t)^2 = \alpha_3,\ (\mathsf{L}_x\mathsf{L}_T\mathsf{M}_x\mathsf{M}_t)^2 = \alpha_4,$ $\mathsf{M}_x^2 = \gamma_1,\ (\mathsf{L}_x\mathsf{M}_x)^2 = \gamma_2,\ \mathsf{M}_t^2 = \beta_1,\ (\mathsf{L}_T\mathsf{M}_t)^2 = \beta_2$ | 84 |
| $Pg_x$ | $\mathbb{Z}_2$ | $L_x, g_x$ | $\mathsf{g}_x\mathsf{L}_x\mathsf{g}_x^{-1}\mathsf{L}_x = \overline{\tau}$ | 2 |
| $Pg_t$ | $\mathbb{Z}_2$ | $L_T, g_t$ | $\mathsf{g}_t\mathsf{L}_T\mathsf{g}_t^{-1}\mathsf{L}_T = \tau$ | 2 |
| $Pg_xg_t$ | $\mathbb{Z}_2^2$ | $g_x, g_t$ | $(\mathsf{g}_x\mathsf{g}_t)^2 = \alpha_1,\ (\mathsf{g}_x\mathsf{g}_t^{-1})^2 = \alpha_2$ | 3 |
| $Pm_xg_t$ | $\mathbb{Z}_2^4$ | $L_T, M_x, g_t$ | $[\mathsf{M}_x : \mathsf{L}_T] = \eta,\ (\mathsf{M}_x\mathsf{g}_t)^2 = \alpha_1,\ (\mathsf{L}_T\mathsf{M}_x\mathsf{g}_t)^2 = \alpha_2,\ \mathsf{M}_x^2 = \gamma$ | 12 |
| $Pm_tg_x$ | $\mathbb{Z}_2^4$ | $L_x, M_t, g_x$ | $[\mathsf{M}_t : \mathsf{L}_x] = \overline{\eta},\ (\mathsf{M}_t\mathsf{g}_x)^2 = \alpha_1,\ (\mathsf{L}_x\mathsf{M}_t\mathsf{g}_x)^2 = \alpha_2,\ \mathsf{M}_t^2 = \beta$ | 12 |
| $Cm_x$ | $\mathbb{Z}_2^2$ | $L_1, L_2, M_x$ | $[\mathsf{L}_1 : \mathsf{L}_2] = \sigma,\ \mathsf{M}_x\mathsf{L}_1\mathsf{M}_x^{-1}\mathsf{L}_2^{-1} = 1,\ \mathsf{M}_x^2 = \gamma$ | 4 |
| $Cm_t$ | $\mathbb{Z}_2^2$ | $L_1, L_2, M_t$ | $[\mathsf{L}_1 : \mathsf{L}_2] = \sigma,\ \mathsf{M}_t\mathsf{L}_1\mathsf{M}_t^{-1}\mathsf{L}_2^{-1} = 1,\ \mathsf{M}_t^2 = \beta$ | 4 |
| $Cm_xm_t$ | $\mathbb{Z}_2^5$ | $L_1, M_x, M_t$ | $(\mathsf{M}_x\mathsf{M}_t)^2 = \alpha_1,\ (\mathsf{L}_1\mathsf{M}_x\mathsf{M}_t)^2 = \alpha_2,\ (\mathsf{L}_1\mathsf{M}_x\mathsf{L}_1^{-1}\mathsf{M}_t)^2 = \alpha_3,\ \mathsf{M}_x^2 = \gamma,\ \mathsf{M}_t^2 = \beta$ | 24 |

TABLE II: $\mathbb{Z}_2$-projective symmetry algebras of 13 $(1,1)$D spacetime groups. All factors take values in $\mathbb{Z}_2$.

The general method to derive all possible nonequivalent $\mathcal{A}$-projective symmetry algebras for $G$ is as follows. First, we choose a presentation $G = \langle \mathcal{S}|\mathcal{R}\rangle = \langle s_1, s_2, ...|r_1(s) = 1, r_2(s) = 1, ...\rangle$. Then we modify the raltions $\mathcal{R}$ into $\widetilde{\mathcal{R}} = \{r_1(s) = \alpha_1, r_2(s) = \alpha_2, ...\}$ by factors $\alpha_1, \alpha_2, ... \in \mathcal{A}$. The remaining task is to determine all possible values of factors $\alpha_i$. From Eq. (11), we see that $\widetilde{G}$ determines a multiplier $\widetilde{\nu}$, which is a function of $n_{a_i}, n_{b_i}, i = 1, 2, ...$, and also a fucntion of $\alpha_1, \alpha_2, ...$. The multiplier $\widetilde{\nu}$ must satisfy the cocycle equation for any three group element $g_a, g_b, g_c$, which leads to a equation involving factors $\alpha_1, \alpha_2, ...$ and parameters $n_{a_i}, n_{b_i}, n_{c_i}, i = 1, 2, ...$. This equation should hold for all possible values of $n_{a_i}, n_{b_i}, n_{c_i}, i = 1, 2, ...$. Its solutions give all possible values of $\alpha_1, \alpha_2, ...$, and thus give us all cohomology classes of projective symmetry algebras. However, if some factors $\alpha_i$ are not cohomology invariants, some solutions may correspond to the same cohomology class. To avoid this situation, we only use cohomology invariants and fix other factors by coboundary transformations at the outset.

While the above cocycle equation method is general, it can be rather tedious. In this paper, we employ a more streamlined approach to identify all possible values of cohomology invariants. Specifically, we use only a small subset of self-consistency conditions derived from the cocycle equation to constrain the cohomology invariants. Since we do not consider all constraints, some of our solutions may be invalid. So to ensure the accuracy of our solutions, we verify them through other means. For $\mathcal{A} = \mathbb{Z}_2$ case, we cross-check our results against the already-known $H^2(G_{st}, \mathbb{Z}_2)$ values. If our findings yield the same number of projective symmetry algebras as $H^2(G_{st}, \mathbb{Z}_2)$, we can validate our results. In the case of $\mathcal{A} = U(1)$, we should cross-check our results against the $H^{2,c}(G_{st}, U(1))$ values. However, for a general wallpaper group, $H^{2,c}(G_{st}, U(1))$ is not available. Fortunately, in most cases, we still have simple method to ensure the correctness of our results. For groups $P1$, $Pm_x$, $Pg_x$ and $Cm_x$, $H^{2,c}(G_{st}, U(1)) = H^2(G_{st}, U(1))$ since they have no anti-unitary operation. So we can cross-check our results with $H^{2,c}(G_{st}, U(1))$ (which are known) in these cases. For groups $P2, Pm_xm_t, Pg_xg_t, Pm_xg_t, Pm_tg_x$ and $Cm_xm_t$, we find that their cohomology invariants can be constrained to be $\mathbb{Z}_2$ value, which means their $U(1)$-projective symmetry algebras are just special cases of $\mathbb{Z}_2$-projective symmetry algebras. Therefore, once we constrain all cohomology invariants to be $\mathbb{Z}_2$ value, we cannot further constrain them and arrive at the final result. For group $Pm_t, Pg_t$ and $Cm_t$, we lack a simple method to verify our results, so we solve the cocyle equation by brute force. After verifying the accuracy of our results for the $U(1)$ cases, we can infer $H^{2,c}(G_{st}, U(1))$ from the possible values of the cohomology invariants.

The above description of our method may seem abstract, so we recommend that readers refer to the examples below, as they can be helpful in clarifying the approach.

### 1. P1

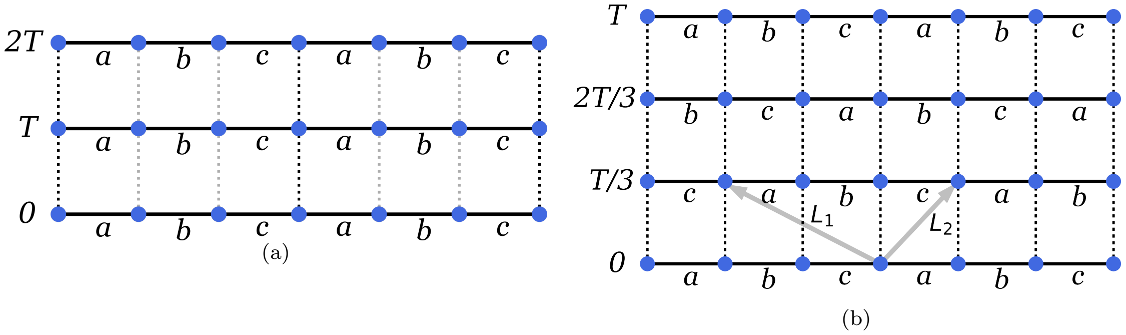


FIG. 1: $P1$ spacetime tight binding model. Hoppings are $T$ periodic. The dashed lines mean variation of hoppings with time. $a, b, c$ are hopping amplitudes at certain times. (a) A spacetime tight binding model with translation symmetry $L_x, L_T$. (b) A spacetime tight binding model with translation symmetry $L_1, L_2$.

The $P1$ spacetime group can be generated by two unit spacetime translations $L_1$ and $L_2$, which are not necessary to be $L_x$ and $L_T$. The two generators commute with each other, $[L_1 : L_2] = L_1L_2L_1^{-1}L_2^{-1} = 1$. So the presentation of $P1$ is

$$P1 = \langle L_1, L_2|[L_1 : L_2]\rangle. \tag{13}$$

Two lattice models with $P1$ symmetry is shown in Fig. 1, one with ordinary spatial and time translation symmetry, another with spacetime translation symmetry.

Projective symmetry algebras can be obtained by modifying the relation by

$$\mathsf{L}_1\mathsf{L}_2\mathsf{L}_1^{-1}\mathsf{L}_2^{-1} = \sigma. \tag{14}$$

For $\mathbb{Z}_2$-projective symmetry algebra, $\sigma$ takes values in $\mathbb{Z}_2 = \{\pm 1\}$, and for $U(1)$-projective symmetry algebra, $\sigma$ takes values in $U(1)$. It is esay to see that $\sigma$ is a cohomology invariant. These results are already consistent with that of group cohomology

$$H^2(P1, \mathbb{Z}_2) = \mathbb{Z}_2, \tag{15}$$

$$H^2(P1, U(1)) = U(1), \tag{16}$$

so the value of the factor $\sigma$ cannot be constrained further.

## 2. P2

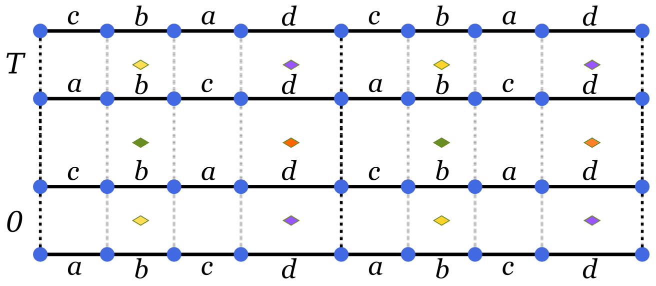


FIG. 2: $P2$ spacetime tight binding model. There are four classes of two-fold rotation centers, marked by diamonds in four colors. Hoppings are centrosymmetric respect to rotation centers.

The $P2$ spacetime group contains two-fold spacetime rotations besides translations. It can be generated by $L_1, L_2$ and spacetime rotation $C = M_x M_t$. The generator $C$ reverses the direction of translation $L_1, L_2$, so the presentation of $P2$ is

$$\begin{aligned} P2 = \quad & \langle L_1, L_2, C | [L_1 : L_2], C L_1 C^{-1} = L_1^{-1}, \\ & C L_2 C^{-1} = L_2^{-1}, C^2 \rangle. \end{aligned} \tag{17}$$

A spacetime tight binding model with $P2$ symmetry is shown in Fig. 2, where we choose $L_1, L_2$ to be $L_x, L_T$ although they can be space-time mixed translations in general. There are four different conjugacy classes of rotations $C_s(R)$, $C_s(L_a C)$, $C_s(L_b C), C_s(L_a L_b C)$, whose rotation centers are shown in Fig. 2 in four different colors. We can recombine the relations to present $P2$ in terms of the squares of four classes of rotations:

$$P2 = \langle L_1, L_2, C | C^2, (L_1 C)^2, (L_2 C)^2, (L_1 L_2 C)^2 \rangle. \tag{18}$$

Projective symmetry algebras can be obtained by modifying the relations by

$$\mathsf{C}^2 = \alpha_1, \tag{19a}$$

$$(\mathsf{L}_1\mathsf{C})^2 = \alpha_2, \tag{19b}$$

$$(\mathsf{L}_2\mathsf{C})^2 = \alpha_3, \tag{19c}$$

$$(\mathsf{L}_1\mathsf{L}_2\mathsf{C})^2 = \alpha_4. \tag{19d}$$

For $\mathbb{Z}_2$-projective symmetry algebras, $\alpha_1, \alpha_2, \alpha_3, \alpha_4 \in \mathbb{Z}_2$ and are cohomology invariants, which is consistent with the result of group cohomology

$$H^2(P2, \mathbb{Z}_2) = \mathbb{Z}_2^4. \tag{20}$$

For $U(1)$-projective symmetry algebras, $\alpha_1, \alpha_2, \alpha_3, \alpha_4$ are also cohomology invariants. The self-consistency conditions require $\alpha_1, \alpha_2, \alpha_3, \alpha_4 \in \mathbb{Z}_2$, which can be seen by

$$(\mathsf{C}^2)\mathsf{C} = \alpha_1\mathsf{C} = \mathsf{C}(\mathsf{C})^2 = \mathsf{C}\alpha_1 = \alpha_1^*\mathsf{C}, \tag{21}$$

and so on. Here we note we used the anti-unitary property of the operator $\mathsf{C} = \mathsf{M}_x\mathsf{M}_t$ and so on.

Although we only use a few self-consistency conditions to constrain the cohomology invariants, once they are all constrained to be $\mathbb{Z}_2$, they cannot be further constrained. Because now the $U(1)$-projective symmetry algebra becomes a $\mathbb{Z}_2$-projective symmetry algebra and we have shown these values of cohomology invariants are allowed for $\mathbb{Z}_2$ case. From the possible values of cohomology invariants, we can infer the twisted group cohomology to be

$$H^{2,c}(P2, U(1)) = \mathbb{Z}_2^4, \tag{22}$$

which is different from the untwisted result $H^2(P2, U(1)) = U(1)$.

### 3. $\mathrm{Pm_x}$

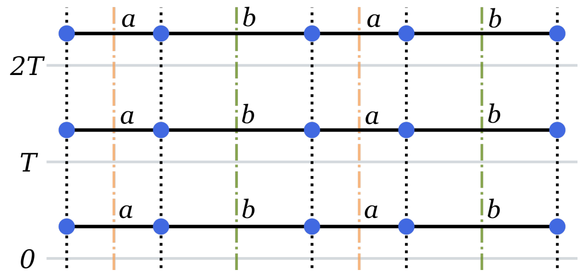


FIG. 3: $Pm_x$ spacetime tight binding model. Mirror axes are plotted as dot-dashed lines. Hoppings are symmetric respect to mirror axes and $T$ periodic.

The $Pm_x$ spacetime group contains space reflections besides translations. The two unit translations must be $L_x, L_T$. The reflection $M_x$ reverses $L_x$ to $L_x^{-1}$ but leaves $L_T$ to be invariant. The presentation can be

$$\begin{aligned} Pm_x = \quad & \langle L_x, L_T, M_x | [L_x : L_T], M_x L_x M_x^{-1} L_x, \\ & M_x L_T M_x^{-1} L_T^{-1}, M_x^2 \rangle. \end{aligned} \tag{23}$$

A spacetime tight binding model with $Pm_x$ symmetry is shown in Fig. 3. There are two different conjugacy classes of mirror reflections $C_s(M_x), C_S(L_x M_x)$, whose reflection axes are shown in Fig. 3 in different colors. The presentation can be rewritten in terms of squares of the two reflections $M_x, L_x M_x$ and their commutators with $L_T$,

$$\begin{aligned} Pm_x = \quad & \langle L_x, L_T, M_x | [M_x : L_T], [L_x M_x : L_T], \\ & M_x^2, (L_x M_x)^2 \rangle. \end{aligned} \tag{24}$$

Projective symmetry algebras can be obtained by modifying the relations by

$$[\mathsf{M}_x : \mathsf{L}_T] = \eta_1, \tag{25a}$$
$$[\mathsf{L}_x\mathsf{M}_x : \mathsf{L}_T] = \eta_2, \tag{25b}$$
$$(\mathsf{M}_x)^2 = \gamma_1, \tag{25c}$$
$$(\mathsf{L}_x\mathsf{M}_x)^2 = \gamma_2. \tag{25d}$$

For $\mathbb{Z}_2$-projective symmetry algebras, $\eta_1, \eta_2, \gamma_1, \gamma_2 \in \mathbb{Z}_2$ and are cohomology invariants.

For $U(1)$-projective symmetry algebras, factors $\gamma_1, \gamma_2$ can be set to be 1 by redefining $\mathsf{L}_x \to \mathsf{L}_x' = \gamma_1^{1/2}\gamma_2^{-1/2}\mathsf{L}_x, \mathsf{M}_x \to \mathsf{M}_x' = \gamma_1^{-1/2}\mathsf{M}_x$. Cohomology invariants $\eta_1, \eta_2 \in \mathbb{Z}_2$, which can be seen by

$$\mathsf{L}_T\gamma_1 = \mathsf{L}_T\mathsf{M}_x^2 = \eta_1^{-2}\mathsf{M}_x^2\mathsf{L}_T = \eta_1^{-2}\gamma_1\mathsf{L}_T. \tag{26}$$
$$\mathsf{L}_T\gamma_2 = \mathsf{L}_T(\mathsf{L}_x\mathsf{M}_x)^2 = \eta_2^{-2}(\mathsf{L}_x\mathsf{M}_x)^2\mathsf{L}_T = \eta_2^{-2}\gamma_2\mathsf{L}_T. \tag{27}$$

These results are consistent with that of the group cohomology

$$H^2(Pm_x, \mathbb{Z}_2) = \mathbb{Z}_2^4, \tag{28}$$
$$H^2(Pm_x, U(1)) = \mathbb{Z}_2^2. \tag{29}$$

### 4. $\mathrm{Pm_t}$

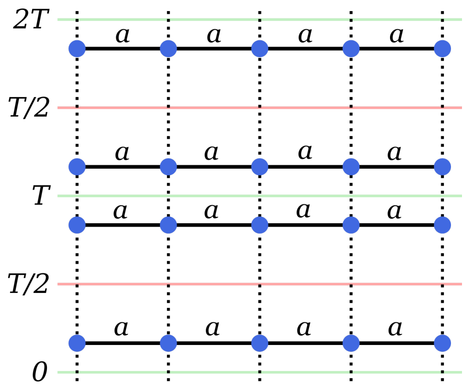


FIG. 4: $Pm_t$ spacetime tight binding model. $nT$ and $nT/2$ are time reversal axes. Hoppings are symmetric respect to these axes and $T$ periodic.

The $Pm_t$ spacetime group contains time reversal besides translations. It can be generated by $L_x, L_T$ and time reversal operator $M_t$. $M_t$ reverses the direction of $L_T$ but leaves $L_x$ invariant, so the presentation can be

$$\begin{aligned} Pm_t = \quad & \langle L_x, L_T, M_t | [L_x : L_T], M_t L_x M_t^{-1} L_x^{-1}, \\ & M_x L_T M_x^{-1} L_T, M_t^2 \rangle. \end{aligned} \tag{30}$$

A spacetime tight binding model with $Pm_t$ symmetry is shown in Fig. 4, where we choose $nT$ and $nT/2$ to be time reversal axes corresponding to two conjugacy classes of time reflections $C_s(M_t), C_s(L_T M_t)$. The presentation can also be rewritten as

$$\begin{aligned} Pm_t = \quad & \langle L_x, L_T, M_t | [L_x : L_T], [M_t : L_x], \\ & M_t^2, (L_T M_t)^2 \rangle. \end{aligned} \tag{31}$$

Projective symmetry algebras can be obtained by modifying the relations by

$$[\mathsf{L}_x : \mathsf{L}_T] = \sigma, \tag{32a}$$
$$[\mathsf{M}_t : \mathsf{L}_x] = \overline{\eta}, \tag{32b}$$
$$(\mathsf{M}_t)^2 = \beta_1, \tag{32c}$$
$$(\mathsf{L}_T \mathsf{M}_t)^2 = \beta_2. \tag{32d}$$

For $\mathbb{Z}_2$-projective symmetry algebras, cohomology invariants $\sigma, \overline{\eta}, \beta_1, \beta_2 \in \mathbb{Z}_2$ , which is consistent with the result of the group cohomology

$$H^2(Pm_t, \mathbb{Z}_2) = \mathbb{Z}_2^4. \tag{33}$$

For $U(1)$-projective symmetry algebras, factor $\overline{\eta}$ can be trivialized by redefining $\mathsf{L}_x \to \mathsf{L}'_x = \overline{\eta}^{1/2}\mathsf{L}_x$. Cohomology invariants $\beta_1, \beta_2 \in \mathbb{Z}_2$ since $\mathsf{M}_t$ and $\mathsf{L}_T\mathsf{M}_t$ are anti-unitary (the proof is similar to Eq. (21)). However, there is no constrain on the cohomology invariant $\sigma$, so $\sigma \in U(1)$. The validity of this result was checked by the general method of cocycle equations, which we do not present here. From the possible values of cohomology invariants, we can infer that

$$H^{2,c}(Pm_t, U(1)) = U(1) \times \mathbb{Z}_2^2. \tag{34}$$

For $\mathbb{Z}_2$-projective symmetry algebras, the projective symmetry algebras can also be written in the form

$$[\mathsf{M}_t : \mathsf{L}_x] = \overline{\eta}_1, \tag{35a}$$
$$[\mathsf{L}_T \mathsf{M}_t : \mathsf{L}_x] = \overline{\eta}_2, \tag{35b}$$
$$(\mathsf{M}_t)^2 = \beta_1, \tag{35c}$$
$$(\mathsf{L}_T \mathsf{M}_t)^2 = \beta_2. \tag{35d}$$

where $\overline{\eta}_1 = \overline{\eta}, \overline{\eta}_2 = \sigma\overline{\eta} \in \mathbb{Z}_2$.

### 5. $\mathrm{Pm_xm_t}$

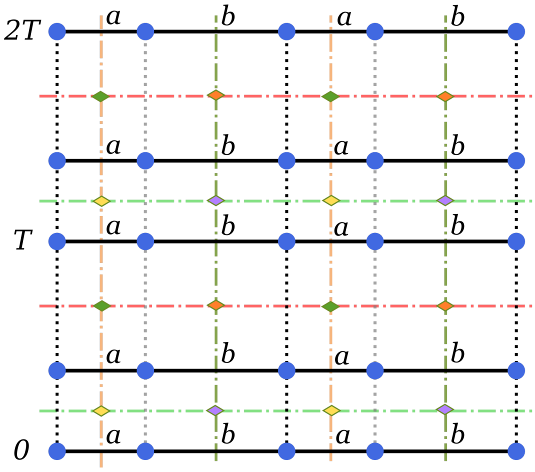


FIG. 5: $Pm_xm_t$ spacetime tight binding model. Mirror axes are plotted as dot-dashed lines, and their intersections are two-fold rotation centers. Hoppings are symmetric respect to mirror axes and $T$ periodic.

The $Pm_xm_t$ spacetime group contains space reflections and time reversal besides translations. It can be generated by $L_x, L_T, M_x, M_t$. The presentation is given by

$$Pm_xm_t = \langle L_x, L_T, M_x, M_t | [L_x, L_T], M_x L_x M_x^{-1} L_x, M_x L_T M_x^{-1} L_T^{-1}, M_t L_x M_t^{-1} L_x^{-1}, M_t L_T M_t^{-1} L_T, M_x^2, M_t^2, [M_x, M_t] \rangle. \tag{36}$$

A spacetime tight binding model with $Pm_xm_t$ symmetry is shown in Fig. 5. There are two classes of spatial mirror axes at $x$ direction and $t$ direction respectively, and their intersections are two-fold rotation centers. The relations can also be expressed in terms of the squares of the four rotations and the four reflections:

$$Pm_xm_t = \langle L_x, L_T, M_x, M_t | (M_x M_t)^2, (L_x M_x M_t)^2, (L_T M_x M_t)^2, (L_x L_T M_x M_t)^2, M_x^2, (L_x M_x)^2, M_t^2, (L_T M_t)^2 \rangle. \tag{37}$$

Projective symmetry algebras can be obtained by modifying the relations by

$$\mathsf{C}^2 = (\mathsf{M}_x \mathsf{M}_t)^2 = \alpha_1, \tag{38a}$$
$$(\mathsf{L}_x \mathsf{C})^2 = \alpha_2, \tag{38b}$$
$$(\mathsf{L}_T \mathsf{C})^2 = \alpha_3, \tag{38c}$$
$$(\mathsf{L}_x \mathsf{L}_T \mathsf{C})^2 = \alpha_4, \tag{38d}$$
$$\mathsf{M}_x^2 = \gamma_1, \tag{38e}$$
$$(\mathsf{L}_x \mathsf{M}_x)^2 = \gamma_2, \tag{38f}$$
$$\mathsf{M}_t^2 = \beta_1, \tag{38g}$$
$$(\mathsf{L}_T \mathsf{M}_t)^2 = \beta_2. \tag{38h}$$

For $\mathbb{Z}_2$-projective symmetry algebras, cohomology invariants $\alpha_1, \alpha_2, \alpha_3, \alpha_4, \gamma_1, \gamma_2, \beta_1, \beta_2 \in \mathbb{Z}_2$, which is consistent with the result of group cohomology

$$H^2(Pm_xm_t, \mathbb{Z}_2) = \mathbb{Z}_2^8. \tag{39}$$

For $U(1)$-projective symmetry algebras, $\gamma_1, \gamma_2$ can be trivialized by redefining $\mathsf{M}_x \to \mathsf{M}'_x = \gamma_1^{-1/2} \mathsf{M}_x, \mathsf{L}_x \to \mathsf{L}'_x = \gamma_2^{-1/2} \gamma_1^{1/2} \mathsf{L}_x$. The cohomology invariants $\alpha_1, \alpha_2, \alpha_3, \alpha_4, \beta_1, \beta_2 \in \mathbb{Z}_2$ due to the anti-unitary property of rotation

and time reversal operators. Since the $U(1)$-projective symmetry algebras have been reduced to special cases of $\mathbb{Z}_2$-projective symmetry algebras, the cohomology invariants cannot be further constrained. We can infer that

$$H^{2,c}(Pm_xm_t, U(1)) = \mathbb{Z}_2^6. \tag{40}$$

### 6. $\mathrm{Pg_x}$

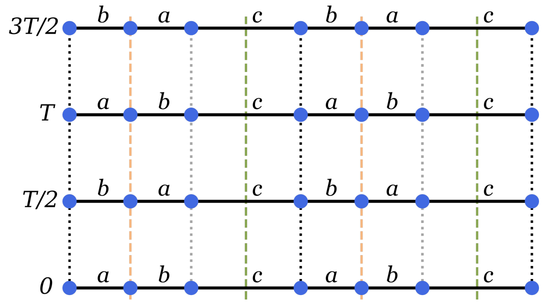


FIG. 6: $Pg_x$ spacetime tight binding model. glide-reflection axes are plotted as dashed lines. Hoppings are glide symmetric respect to these axes.

Besides translations, the $Pg_x$ spacetime group contains a glide reflection operation $g_x$, which is a reflection at $x$ direction followed by a $T/2$ translation at $t$ direction. Since $L_T = g_x^2$, we can take $L_x, g_x$ as generators. $g_x$ reverses the direction of $L_x$, so the presentation can be given by

$$Pg_x = \langle L_x, g_x | g_x L_x g_x^{-1} L_x \rangle. \tag{41}$$

A spacetime tight binding model is shown in Fig. 6. There are two classes of glide-reflection axes, which are shown in different colors.

Projective symmetry algebras can be obtained by modifying the relation by

$$\mathsf{g}_x \mathsf{L}_x \mathsf{g}_x^{-1} \mathsf{L}_x = \overline{\tau}. \tag{42}$$

For $\mathbb{Z}_2$-projective symmetry algebras, cohomology invariant $\overline{\tau} \in \mathbb{Z}_2$, while for $U(1)$-projective symmetry algebras, $\overline{\tau}$ can be trivialized by redefining $\mathsf{L}_x \to \mathsf{L}_x' = \overline{\tau}^{-1/2} \mathsf{L}_x$. These results are consistent with that of the group cohomology

$$H^2(Pg_x, \mathbb{Z}_2) = \mathbb{Z}_2, \tag{43}$$
$$H^2(Pg_x, U(1)) = 1. \tag{44}$$

### 7. $\mathrm{Pg_t}$

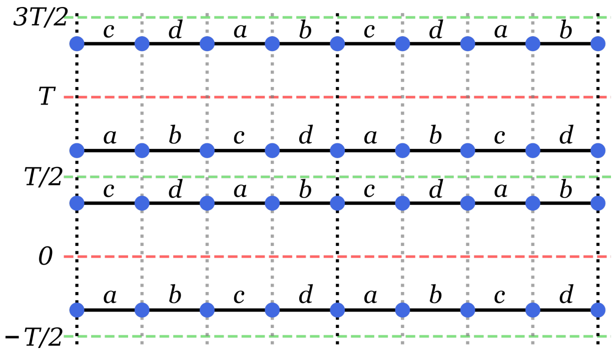


FIG. 7: $Pg_t$ spacetime tight binding model. glide-reflection axes are plotted as dashed lines. Hoppings are glide symmetric respect to these axes and $T$ periodic.

Besides translations, the $Pg_t$ spacetime group contains a glide reflection operation $g_t$, which is a reflection at $t$ direction followed by a half translation at $x$ direction, i.e., $g_t = L_{x/2}M_t$. Since $L_x = g_t^2$, we can take $L_T, g_t$ as generators. $g_t$ reverses the direction of $L_T$, so the presentation can be given by

$$Pg_t = \langle L_T, g_t | g_t L_T g_t^{-1} L_T \rangle. \tag{45}$$

A spacetime tight binding model is shown in Fig. 7. There are two classes of glide-reflection axes, which are shown in different colors.

Projective symmetry algebras can be obtained by modifying the relation by

$$\mathsf{g}_t \mathsf{L}_T \mathsf{g}_t^{-1} \mathsf{L}_T = \tau. \tag{46}$$

For $\mathbb{Z}_2$-projective symmetry algebras, cohomology invariant $\tau \in \mathbb{Z}_2$, which is consistent with the result of group cohomology

$$H^2(Pg_t, \mathbb{Z}_2) = \mathbb{Z}_2. \tag{47}$$

For $U(1)$-projective symmetry algebras, cohomology invariant $\tau \in U(1)$. One can check this result by the general method of cocycle equation. From this result, we infer that

$$H^{2,c}(Pg_t, U(1)) = U(1). \tag{48}$$

### 8. $\mathrm{Pg_xg_t}$

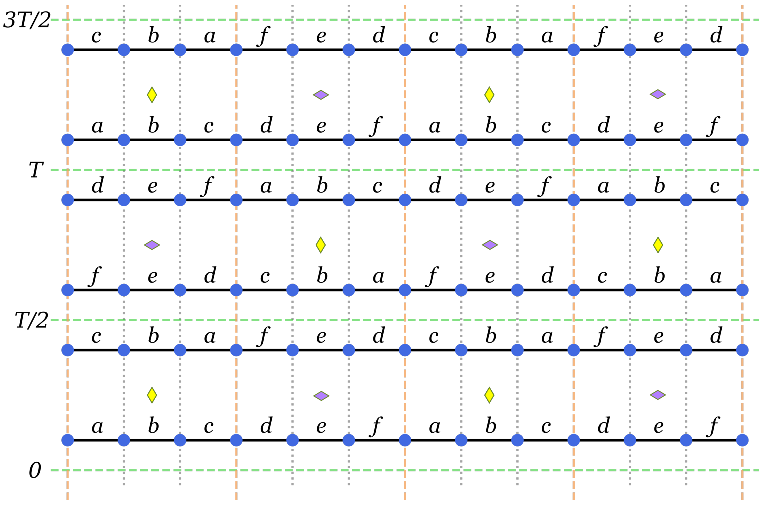


FIG. 8: $Pg_xg_t$ spacetime tight binding model. glide-reflection axes are plotted as dashed lines. Hoppings are glide symmetric respect to these axes. Two-fold rotation centers are plotted as diamonds.

The $Pg_xg_t$ spacetime group contains glide reflections at both $x$ and $t$ directions. Since $g_x^2 = L_T, g_t^2 = L_x$, the generators can be chosen as $g_x, g_t$. The combination operations $g_xg_t$ and $g_xg_t^{-1}$ are two-fold rotations. The presentation can be written as

$$Pg_xg_t = \quad \langle g_x, g_t | (g_xg_t)^2, (g_xg_t^{-1})^2 \rangle. \tag{49}$$

A spacetime tight binding model with $Pg_xg_t$ symmetry is shown in Fig. 8. There are two classes two-fold rotation centers corresponding to $C_s(g_xg_t)$ and $C_s(g_xg_t^{-1})$ respectively.

Projective symmetry algebras can be obtained by modifying the relations by

$$(\mathsf{g}_x\mathsf{g}_t)^2 = \alpha_1, \tag{50a}$$
$$(\mathsf{g}_x\mathsf{g}_t^{-1})^2 = \alpha_2. \tag{50b}$$

For $\mathbb{Z}_2$-projective symmetry algebras, cohomology invariants $\alpha_1, \alpha_2 \in \mathbb{Z}_2$, which is consistent with the result of group cohomology

$$H^2(Pg_xg_t, \mathbb{Z}_2) = \mathbb{Z}_2^2. \tag{51}$$

For $U(1)$-projective symmetry algebras, cohomology invariants $\alpha_1, \alpha_2 \in \mathbb{Z}_2$, which is due to the anti-unitary property of $\mathsf{g}_x\mathsf{g}_t$ and $\mathsf{g}_x\mathsf{g}_t^{-1}$. Since the $U(1)$-projective symmetry algebras have been reduced to $\mathbb{Z}_2$-projective symmetry algebras, $\alpha_1$ and $\alpha_2$ cannot be constrained further. From this result, we can infer that

$$H^{2,c}(Pg_xg_t, U(1)) = \mathbb{Z}_2^2. \tag{52}$$

### 9. $\mathrm{Pm_xg_t}$

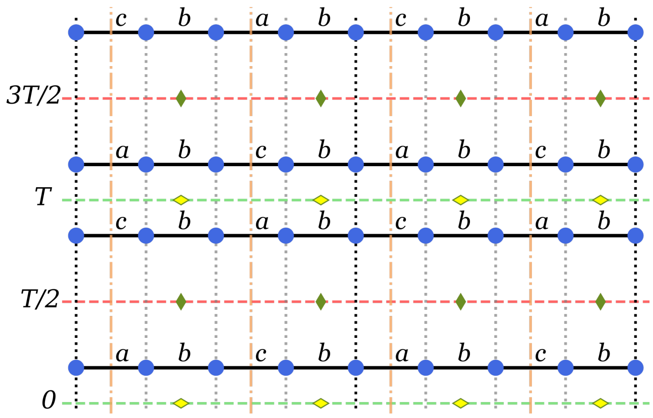


FIG. 9: $Pm_xg_t$ spacetime tight binding model. glide-reflection axes are plotted as dashed lines. Mirror axes are plotted as dot-dashed lines. Two-fold rotation centers are plotted as diamonds. Hoppings are glide symmetric respect to glide-reflection axes and symmetric respect to mirror axes.

The $Pm_xg_t$ spacetime group contains reflections at $x$ direction and glide-reflections at $t$ direction. It can be generated by $L_T, M_x, g_t$. The presentation can be given by

$$\begin{aligned} Pm_xg_t = \quad & \langle L_T, M_x, g_t, | M_xL_TM_x^{-1}L_T^{-1}, g_tL_Tg_t^{-1}L_y, \\ & M_xg_tM_x^{-1}g_t, M_x^2\rangle. \end{aligned} \tag{53}$$

A spacetime tight binding model with $Pm_xg_t$ symmetry is shown in Fig. 9. There is one class of glide reflection axes, and two classes of time mirror axes, also there are two classes of two-fold rotation centers, corresponding to $C_s(M_xg_t)$ and $C_s(L_TM_xg_t)$ respectively. We can also rewrite the presentation in terms of the commutator $[M_x : L_T]$ and the squares of rotations and reflection,

$$\begin{aligned} Pm_xg_t = \quad & \langle L_T, M_x, g_t | [M_x : L_T], (M_xg_t)^2, \\ & (L_TM_xg_t)^2, M_x^2\rangle. \end{aligned} \tag{54}$$

Projective symmetry algebras can be obtained by modifying the relations by

$$\mathsf{M}_x\mathsf{L}_T\mathsf{M}_x^{-1}\mathsf{L}_T^{-1} = \eta \tag{55a}$$
$$(\mathsf{M}_x\mathsf{g}_t)^2 = \alpha_1, \tag{55b}$$
$$(\mathsf{L}_T\mathsf{M}_x\mathsf{g}_t)^2 = \alpha_2, \tag{55c}$$
$$\mathsf{M}_x^2 = \gamma. \tag{55d}$$

For $\mathbb{Z}_2$-projective symmetry algebras, cohomology invariants $\eta, \alpha_1, \alpha_2, \gamma \in \mathbb{Z}_2$, which is consistent with the result of group cohomology

$$H^2(Pm_xg_t, \mathbb{Z}_2) = \mathbb{Z}_2^4. \tag{56}$$

For $U(1)$-projective symmetry algebras, factor $\gamma$ can be trivialized by redefining $\mathsf{M}_x \to \mathsf{M}'_x = \gamma^{-1/2}\mathsf{M}_x$, and cohomology invariants $\alpha_1, \alpha_2 \in \mathbb{Z}_2$ due to the anti-unitary property of $\mathsf{M}_x\mathsf{g}_t$ and $\mathsf{L}_T\mathsf{M}_x\mathsf{g}_t$. Cohomology invariants $\eta \in \mathbb{Z}_2$, which can be seen by

$$\mathsf{L}_T\gamma = \mathsf{L}_T\mathsf{M}_x^2 = \eta^{-2}\mathsf{M}_x^2\mathsf{L}_T = \eta^{-2}\gamma\mathsf{L}_T. \tag{57}$$

Since the $U(1)$-projective symmetry algebras have been reduced to special cases of $\mathbb{Z}_2$-projective symmetry algebras, the cohomology invariants $\alpha_1, \alpha_2, \eta$ cannot be further constrained. We can infer that

$$H^{2,c}(Pm_xg_t, U(1)) = \mathbb{Z}_2^3. \tag{58}$$

### 10. $\mathrm{Pm_tg_x}$

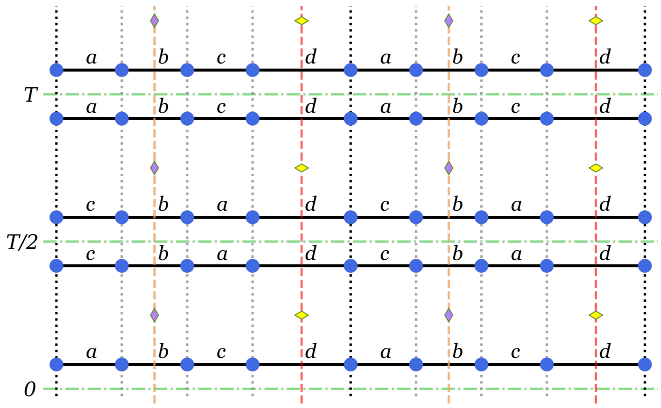


FIG. 10: $Pm_tg_x$ spacetime tight binding model. glide-reflection axes are plotted as dashed lines. Mirror axes are plotted as dot-dashed lines. Two-fold rotation centers are plotted as diamonds. Hoppings are glide symmetric respect to glide-reflection axes and symmetric respect to mirror axes.

The $Pm_tg_x$ spacetime group contains reflections at $t$ direction and glide-reflections at $x$ direction. Its generators can be chosen as $L_x, M_t, g_x$. The presentation can be given by

$$\begin{aligned} Pm_tg_x = \quad & \langle L_x, M_t, g_x, | M_tL_xM_t^{-1}L_x^{-1}, g_xL_xg_x^{-1}L_x, \\ & M_tg_xM_t^{-1}g_x, M_t^2\rangle. \end{aligned} \tag{59}$$

A spacetime tight binding model with $Pm_tg_x$ symmetry is shown in Fig. 10. There is one class of glide-reflection axes and two classes of spatial mirror axes, also there are two classes of two-fold rotation centers, corresponding to $C_s(M_tg_x)$ and $C_s(L_xM_tg_x)$ respectively. We can also rewrite the presentation in terms of the commutator $[M_t : L_x]$ and the squares of rotations and reflection,

$$\begin{aligned} Pm_tg_x = \quad & \langle L_x, M_t, g_x | [M_t : L_x], (M_tg_x)^2, \\ & (L_xM_tg_x)^2, M_t^2\rangle. \end{aligned} \tag{60}$$

Projective symmetry algebras can be obtained by modifying the relations by

$$\mathsf{M}_t\mathsf{L}_x\mathsf{M}_t^{-1}\mathsf{L}_x^{-1} = \overline{\eta} \tag{61a}$$
$$(\mathsf{M}_t\mathsf{g}_x)^2 = \alpha_1, \tag{61b}$$
$$(\mathsf{L}_x\mathsf{M}_t\mathsf{g}_x)^2 = \alpha_2, \tag{61c}$$
$$\mathsf{M}_t^2 = \beta. \tag{61d}$$

For $\mathbb{Z}_2$-projective symmetry algebras, cohomology invariants $\overline{\eta}, \alpha_1, \alpha_2, \beta \in \mathbb{Z}_2$, which is consistent with the result of group cohomology

$$H^2(Pm_xg_t, \mathbb{Z}_2) = \mathbb{Z}_2^4. \tag{62}$$

For $U(1)$-projective symmetry algebras, factor $\overline{\eta}$ can be trivialized by redefining $\mathsf{L}_x \to \mathsf{L}'_x = \overline{\eta}^{1/2}\mathsf{L}_x$, and cohomology invariants $\alpha_1, \alpha_2, \beta \in \mathbb{Z}_2$ due to the anti-unitary property of $\mathsf{M}_x\mathsf{g}_t, \mathsf{L}_T\mathsf{M}_x\mathsf{g}_t, \mathsf{M}_t$. Since the $U(1)$-projective symmetry algebras have been reduced to special cases of $\mathbb{Z}_2$-projective symmetry algebras, the cohomology invariants $\alpha_1, \alpha_2, \beta$ cannot be further constrained. We can infer that

$$H^{2,c}(Pm_tg_x, U(1)) = \mathbb{Z}_2^3. \tag{63}$$

### 11. $\mathrm{Cm_x}$

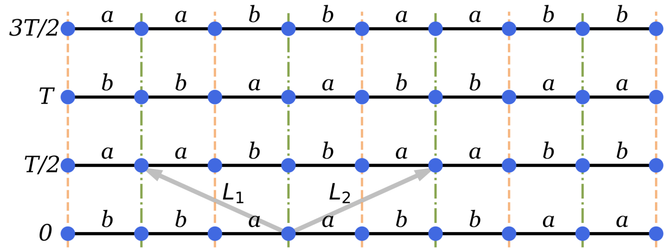


FIG. 11: $Cm_x$ spacetime tight binding model. $L_1$ and $L_2$ are two space-time translations. Mirror axes are plotted as dot-dashed lines. Hoppings are symmetric respect to mirror axes and translation invariant under $L_1$ and $L_2$.

The $Cm_x$ spacetime group contains mirror reflection $M_x$, which interchanges the two unit translations $L_1, L_2$. Since the time direction and space direction is inequivalent, $L_1, L_2$ must be spacetime mixed. The presentation can be given by

$$Cm_x = \langle L_1, L_2, M_x | [L_1 : L_2], M_xL_1M_x^{-1}L_2^{-1}, M_x^2 \rangle. \tag{64}$$

A spacetime tight binding model with $Cm_x$ symmetry is shown in Fig. 11. There are two classes of mirror axes. Projective symmetry algebras can be obtained by modifying the relations by

$$\mathsf{L}_1\mathsf{L}_2\mathsf{L}_1^{-1}\mathsf{L}_2^{-1} = \sigma, \tag{65a}$$
$$\mathsf{M}_x\mathsf{L}_1\mathsf{M}_x^{-1}\mathsf{L}_2^{-1} = \eta, \tag{65b}$$
$$\mathsf{M}_x^2 = \gamma. \tag{65c}$$

For $\mathbb{Z}_2$-projective symmetry algebras, $\eta$ can be trivialized by redefining $\mathsf{L}_1 \to \mathsf{L}'_1 = \eta^{-1}\mathsf{L}_1$, and cohomology invariants $\sigma, \gamma \in \mathbb{Z}_2$.

For $U(1)$-projective symmetry algebras, $\eta, \gamma$ can be trivialized by redefining $\mathsf{L}_1 \to \mathsf{L}'_1 = \eta^{-1}\mathsf{L}_1, \mathsf{M}_x \to \mathsf{M}'_x = \gamma^{-1/2}\mathsf{M}_x$. Cohomology invariant $\sigma \in \mathbb{Z}_2$ due to the self-consistency condition required by the mirror reflection:

$$\mathsf{M}_x\sigma = \mathsf{M}_x\mathsf{L}_1\mathsf{L}_2\mathsf{L}_1^{-1}\mathsf{L}_2^{-1} = \mathsf{L}_2\mathsf{L}_1\mathsf{L}_2^{-1}\mathsf{L}_1^{-1}\mathsf{M}_x = \mathsf{M}_x\sigma^{-1}. \tag{66}$$

These results are consistent with that of the group cohomology

$$H^2(Cm_x, \mathbb{Z}_2) = \mathbb{Z}_2^2, \tag{67}$$
$$H^2(Cm_x, U(1)) = \mathbb{Z}_2. \tag{68}$$

### 12. $\mathrm{Cm_t}$

The $Cm_t$ spacetime group contains mirror reflection $M_t$, which interchanges two space-time translations $L_1, L_2$. Since the time direction and space direction is inequivalent, $L_1, L_2$ must be spacetime mixed. The presentation can be given by

$$Cm_t = \langle L_1, L_2, M_t | [L_1 : L_2], M_tL_1M_t^{-1}L_2^{-1}, M_t^2 \rangle. \tag{69}$$

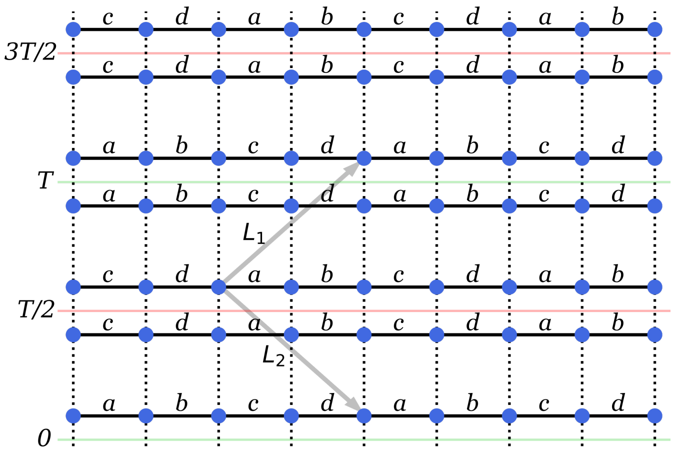


FIG. 12: $Cm_t$ spacetime tight binding model. $L_1$ and $L_2$ are two translation elements. $nT/2$ are time reversal axes. Hoppings are symmetric respect to these axes and translation invariant under $L_1$ and $L_2$. We plot a set of hoppings which are related by translations or time reversals.

A spacetime tight binding model with $Cm_t$ symmetry is shown in Fig. 12. There are two classes of time reversal axes.

Projective symmetry algebras can be obtained by modifying the relations by

$$\mathsf{L}_1\mathsf{L}_2\mathsf{L}_1^{-1}\mathsf{L}_2^{-1} = \sigma, \tag{70a}$$
$$\mathsf{M}_t\mathsf{L}_1\mathsf{M}_t^{-1}\mathsf{L}_2^{-1} = \eta, \tag{70b}$$
$$\mathsf{M}_t^2 = \beta. \tag{70c}$$

For $\mathbb{Z}_2$-projective symmetry algebras, $\eta$ can be trivialized by redefining $\mathsf{L}_1 \to \mathsf{L}_1' = \eta\mathsf{L}_1$, and cohomology invariants $\sigma, \beta \in \mathbb{Z}_2$. This result is consistent with that of the group cohomology

$$H^2(Cm_t, \mathbb{Z}_2) = \mathbb{Z}_2^2. \tag{71}$$

For $U(1)$-projective symmetry algebras, $\eta$ can also be trivialized by redefining $\mathsf{L}_1 \to \mathsf{L}_1' = \eta\mathsf{L}_1$. Cohomology invariant $\beta \in \mathbb{Z}_2$ due to the anti-unitary property of $\mathsf{M}_t$. There is no constrain on the cohomology invariant $\sigma$, so $\sigma \in U(1)$. This result can be checked by the general method of cocycle equation. From the possible values of cohomology invariants, we can infer that

$$H^{2,c}(Cm_t, U(1)) = U(1) \times \mathbb{Z}_2. \tag{72}$$

### 13. $\mathrm{Cm_xm_t}$

The $Cm_xm_t$ spacetime group is generated by $L_1, L_2, M_x, M_t$. $L_1, L_2$ must be spacetime mixed. Both $M_x$ and $M_t$ interchange $L_1$ and $L_2$. The presentation can be given by

$$\begin{aligned} Cm_xm_t = \; & \langle L_1, L_2, M_x, M_t | [L_1 : L_2], M_xL_1M_x^{-1}L_2, \\ & M_tL_1M_t^{-1}L_2^{-1}, [M_x : M_t], M_x^2, M_t^2 \rangle. \end{aligned} \tag{73}$$

A spacetime tight binding model with $Cm_xm_t$ symmetry is shown in Fig. 13. There are two classes of time reversal axes and two classes of spatial reflection axes. There are also three classes of two-fold rotation centers, corresponding to $C_s(M_xM_t), C_s(L_1M_xM_t), C_s(L_1M_xL_1^{-1}M_t)$ respectively. We can rewrite the presentation in terms of squares of rotations and reflections,

$$\begin{aligned} Cm_xm_t = \; & \langle L_1, M_x, M_t | (M_xM_t)^2, (L_1M_xM_y)^2, \\ & (L_1M_xL_1^{-1}M_t)^2, M_x^2, M_t^2 \rangle. \end{aligned} \tag{74}$$

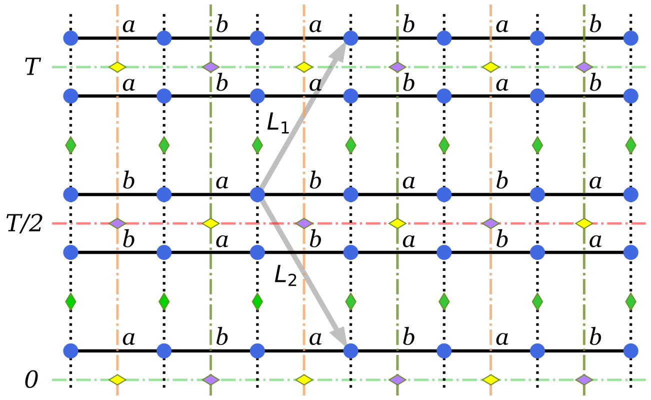


FIG. 13: $Cm_xm_t$ spacetime tight binding model. $L_1$ and $L_2$ are two space-time translations. Mirror axes are plotted as dot-dashed lines. Hoppings are symmetric respect to these axes and translation invariant under $L_1$ and $L_2$. Two-fold rotation centers are plotted as diamonds. We plot a set of hoppings which are related by translations or mirror reflections.

Projective symmetry algebras can be obtained by modifying the relations by

$$\mathsf{C}^2 = (\mathsf{M}_x\mathsf{M}_t)^2 = \alpha_1, \tag{75a}$$
$$(\mathsf{L}_1\mathsf{C})^2 = (\mathsf{L}_1\mathsf{M}_x\mathsf{M}_t)^2 = \alpha_2, \tag{75b}$$
$$(\mathsf{L}_1\mathsf{L}_2\mathsf{C})^2 = (\mathsf{L}_1\mathsf{M}_x\mathsf{L}_1^{-1}\mathsf{M}_t)^2 = \alpha_3, \tag{75c}$$
$$\mathsf{M}_x^2 = \gamma, \tag{75d}$$
$$\mathsf{M}_t^2 = \beta. \tag{75e}$$

For $\mathbb{Z}_2$-projective symmetry algebras, cohomology invariants $\alpha_1, \alpha_2, \alpha_3, \gamma, \beta \in \mathbb{Z}_2$, which is consistent with the result of group cohomology

$$H^2(Cm_xm_t, \mathbb{Z}_2) = \mathbb{Z}_2^5. \tag{76}$$

For $U(1)$-projective symmetry algebras, factor $\gamma$ can be trivialized by redefining $\mathsf{M}_x \to \mathsf{M}'_x = \gamma^{-1/2}\mathsf{M}_x$. Cohomology invariants $\alpha_1, \alpha_2, \alpha_3, \beta \in \mathbb{Z}_2$ due to the anti-unitary property of $\mathsf{M}_x\mathsf{M}_t, \mathsf{L}_1\mathsf{M}_x\mathsf{M}_t, \mathsf{L}_1\mathsf{M}_x\mathsf{L}_1^{-1}\mathsf{M}_t$ and $\mathsf{M}_t$. Since the $U(1)$-projective symmetry algebras have been reduced to special cases of $\mathbb{Z}_2$-projective symmetry algebras, the cohomology invariants $\alpha_1, \alpha_2, \alpha_2, \beta$ cannot be further constrained. We can infer that

$$H^{2,c}(Cm_xm_t, U(1)) = \mathbb{Z}_2^4. \tag{77}$$

### C. Time crystals with gauge structures

In this section, we present a formalism for studying projective symmetries of time crystals with gauge structures. One interesting feature of this formalism is that cohomology invariants can be interpreted in terms of flux, enabling us to realize different projective symmetry algebras by tuning the flux. Different from the magnetic flux which makes crystal symmetries projectively represented, here the flux makes spacetime crystalline symmetries projectively represented is *electric flux*. While magnetic flux is more commonly known, electric flux may be less familiar to some readers. Therefore, we provide a brief introduction to electric flux before proceeding further.

#### 1. Electric A-B effect and electric flux

In the seminal paper by Aharonov and Bohm (55), they raised two types of A-B effects: electric A-B effect and magnetic A-B effect. While the latter is well-known, the former gets less attention, which is partly due to the difficulties to observe it. Although the type-II electric A-B effect has been confirmed by experiments (56-58), the type-I electric A-B effect which requires the particle to experience a vanishing field is still lack of observation.

In general, when an electron circles a spacetime loop $C$, it acquires an A-B phase $e^{i\Delta g}$,

$$\Delta g = \frac{e}{\hbar}\oint_C A_\mu(x)dx^\mu, \tag{78}$$

where $A_\mu = (-\phi, \vec{A})$. By applying Stokes' theorem, we can write it as

$$\Delta g = \pm\frac{e}{\hbar}\int_S \frac{1}{2}F_{\mu\nu}dx^\mu \wedge dx^\nu, \tag{79}$$

where $S$ is an area whose boundary is $C$ and the sign depends on the direction of $C$. When the loop is in a spatial plane, this formula gives us the well-known magnetic A-B phase. But when the loop is in a spacetime plane, for example the $t-x$ plane, it gives us an electric A-B phase

$$\Delta g = \pm\frac{e}{\hbar}\int_S E_x dt dx = \pm\frac{e}{\hbar}\Phi_E, \tag{80}$$

where $\Phi_E$ is called electric flux.

In this paper, we focus on (1,1)D spacetime lattice systems, where the electric flux is solely induced by $E_x$. Consider a spacetime plaquette with four vertex $(x_1,t_1),(x_2,t_1),(x_2,t_2),(x_1,t_2)$. The electric flux on it is

$$\Phi_E = \int_{x_1}^{x_2} A_x(x,t_1)dx - \int_{t_1}^{t_2}\phi(x_2,t)dt - \int_{x_1}^{x_2} A_x(x,t_2)dx + \int_{t_1}^{t_2}\phi(x_1,t)dt. \tag{81}$$

In this paper, we always adopt the gauge $\phi = 0$, i.e., $E_x = -\partial A_x/\partial t$. With this gauge, the above flux

$$\Phi_E = \int_{x_1}^{x_2} A_x(x,t_1)dx - \int_{x_1}^{x_2} A_x(x,t_2)dx. \tag{82}$$

### 2. Symmetries of spacetime tight binding models with gauge structures

In this paper, we study (1,1)D spacetime tight-binding models, which can be given by the Hamiltonian

$$H(t) = \sum_{\langle ij\rangle} w_{ij}(t)|i\rangle\langle j| = \sum_{\langle ij\rangle} |w_{ij}(t)|e^{iA_{ij}(t)}|i\rangle\langle j|, \tag{83}$$

where the phase $A_{ij}(t)$ can be seen as induced by a guage field, $A_{ij}(t) = -\int_i^j A_x(x,t)dx$ (we take $e=\hbar=1$). For a spacetime loop $(i,t_1)\to(i+1,t_1)\to(i+1,t_2)\to(i,t_2)\to(i,t_1)$, the electric flux on it is

$$\Phi = -(A_{i,i+1}(t_1) - A_{i,i+1}(t_2)). \tag{84}$$

In general, a spacetime symmetry operation $R$ that preserves the lattice (strengths of hoppings) and flux configuration may change the gauge configuration (phase $A_{ij}(t)$). The transformed gauge configuration is related to the original configuration by a gauge transformation $\mathsf{G}_R$, since they correspond to the same flux configuration. Therefore, the *proper* spacetime symmetry operator should be

$$\mathsf{R} = \mathsf{G}_R R. \tag{85}$$

The action of $\mathsf{R}$ on $H(t)$ is given by

$$\begin{aligned}
\mathsf{R}H(t)\mathsf{R}^{-1} &= \sum_{ij}\widetilde{R}(w_{ij}(R^{-1}t))\mathsf{G}_R|R(i)\rangle\langle R(j)|\mathsf{G}_R^{-1} && (86)\\
&= \sum_{ij}\widetilde{R}(w_{ij}(R^{-1}t))\mathsf{G}_R(R(i))\mathsf{G}_R^{-1}(R(j))|R(i)\rangle\langle R(j)| \\
&= \sum_{ij}\mathsf{G}_R(i)\mathsf{G}_R^{-1}(j)\widetilde{R}(w_{R^{-1}(i)R^{-1}(j)}(R^{-1}t))|i\rangle\langle j|, && (87)
\end{aligned}$$

where $\widetilde{R}$ is the complex conjugate if $R$ contains time reversal, $R(i), R(t)$ is defined as $(R(i), R(t)) = R(i,t)$, and $\mathsf{G}_R(i)$ is the phase of gauge transformation on site $i$. The Hamiltonian $H(t)$ is invariant under $\mathsf{R}$ if the following condition is satisfied:

$$\mathsf{G}_R(i)\mathsf{G}_R^{-1}(j)\widetilde{R}(w_{R^{-1}(i)R^{-1}(j)}(R^{-1}t)) = w_{ij}. \tag{88}$$

This formula will help us derive the flux interpretation of cohomology invariants in the next section.

Now, we prove the claim in main text that $\Omega(R_1,R_2) = \mathsf{G}_{R_1}R_1\mathsf{G}_{R_2}R_1^{-1}\mathsf{G}_{R_1R_2}^{-1}$ is a $U(1)$ factor. First we observe that $\Omega(R_1,R_2)$ is a pure gauge transformation, i.e., a diagonal matrix with $i$th diagonal entry being $\mathsf{G}_{R_1}(i)\mathsf{G}_{R_2}(R_1^{-1}(i))/\mathsf{G}_{R_1R_2}(i)$. It commutes with all possible symmetry-preserving Hamiltonian. If we presume the Hamiltonian is a connected lattice model, $\Omega(R_1,R_2)$ will be proportional to the identity matrix, namely $[\Omega(R_1,R_2)]_{ij} = \nu(R_1,R_2)\delta_{ij}$ with $\nu(R_1,R_2)\in U(1)$.

### 3. Flux interpretation of cohomology invariants

In Table. I and Table. II, there are five types of cohomology invariants:
(1) Cohomology invariants of translation subgroups, which we denote by $\sigma$.
(2) Cohomology invariants of rotations, which we denote by $\alpha$.
(3) Cohomology invariants between translations and reflections. We denote the cohomology invariant between $\mathsf{L}_x$ and $\mathsf{M}_t$ by $\eta$, and the cohomology invariant between $\mathsf{L}_T$ and $\mathsf{M}_x$ by $\overline{\eta}$ (which can be nontrivial only for $\mathbb{Z}_2$-projective symmetry algebras).
(4) Cohomology invariants between translations and glide-reflections. We denote the cohomology invariant between $\mathsf{L}_T$ and $\mathsf{g}_t$ by $\tau$, and the cohomology invariant between $\mathsf{L}_x$ and $\mathsf{g}_x$ by $\overline{\tau}$ (which can be nontrivial only for $\mathbb{Z}_2$-projective symmetry algebras).
(5) Cohomology invariants of reflections. We denote the cohomology invariants of time reversals by $\beta$, and the cohomolgy invariants of spatial reflections by $\gamma$ (which can be nontrivial only for $\mathbb{Z}_2$-projective symmetry algebras).
As we will see, cohomology invariants can be interpretated in terms of fluxes.

#### i. *Cohomology invariants of translation subgroups*

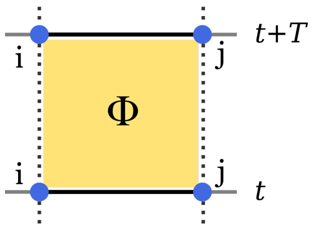


FIG. 14: Flux interpretation of the cohomology invariants of translation subgroups. This lattice has $\mathsf{L}_x$ and $\mathsf{L}_T$ symmetry, and site $j = L_x(i)$.

For the translation subgroup, the projective algebraic relation $\mathsf{L}_1\mathsf{L}_2\mathsf{L}_1^{-1}\mathsf{L}_2 = \sigma$ requires that

$$\begin{aligned} \mathsf{L}_1\mathsf{L}_2\mathsf{L}_1^{-1}\mathsf{L}_2^{-1}f(t)|i\rangle &= \mathsf{G}_1L_1\mathsf{G}_2L_2(\mathsf{G}_1L_1)^{-1}(\mathsf{G}_2L_2)^{-1}f(t)|i\rangle \\ &= \mathsf{G}_1(i)\mathsf{G}_2(L_1^{-1}(i))\mathsf{G}_1^*(L_2^{-1}(i))\mathsf{G}_2^*(i)f(t)|i\rangle \quad (89) \\ &= \sigma f(t)|i\rangle, \quad (90) \end{aligned}$$

which means that the gauge transformations on sites satisfy

$$\mathsf{G}_1(i)\mathsf{G}_2(L_1^{-1}(i))\mathsf{G}_1^*(L_2^{-1}(i))\mathsf{G}_2^*(i) = \sigma. \quad (91)$$

First, let us consider the translation group generated by $\mathsf{L}_x$ and $\mathsf{L}_T$ with $\mathsf{L}_x\mathsf{L}_T\mathsf{L}_x^{-1}\mathsf{L}_T^{-1} = \sigma$. Eq. (96) becomes

$$\mathsf{G}_T(L_x^{-1}(i))\mathsf{G}_T^*(i) = \sigma. \quad (92)$$

A lattice with $\mathsf{L}_x$ and $\mathsf{L}_T$ symmetry is shown in Fig. 14, where $i = L_x^{-1}(j)$. There can be some sites between $i$ and $j$ in general, and we define

$$e^{A_{ij}(t)} = e^{A_{i,i+1}(t)}e^{A_{i+1,i+2}(t)}\cdots e^{A_{j-1,j}(t)}. \quad (93)$$

For a general symmetry operator $\mathsf{R}$, using Eq. (88) for every hopping between site $i$ and $j$, we get

$$\mathsf{G}_R(i)\mathsf{G}_R^{-1}(j)\widetilde{R}(e^{iA_{R^{-1}(i)R^{-1}(j)}(R^{-1}t)}) = e^{iA_{ij}(t)}. \quad (94)$$

Take $\mathsf{R} = \mathsf{L}_T$, we have

$$e^{iA_{ij}(t)}e^{-iA_{ij}(t+T)} = \mathsf{G}_T^{-1}(i)\mathsf{G}_T(j) = (\mathsf{G}_T(L_x^{-1}(j))\mathsf{G}_T^*(j))^{-1} = \sigma^{-1}. \quad (95)$$

The left-hand side is exactly $e^{-i\Phi}$, where $\Phi$ is the electric flux in the loop $\mathsf{L}_x\mathsf{L}_T\mathsf{L}_x^{-1}\mathsf{L}_T^{-1}$, so we have a flux interpretation for the cohomology invariant $\sigma$,

$$\sigma = e^{i\Phi}. \quad (96)$$

We then consider a general translation group generated by $\mathsf{L}_1, \mathsf{L}_2$ with $\mathsf{L}_1\mathsf{L}_2\mathsf{L}_1^{-1}\mathsf{L}_2 = \sigma$, where $\mathsf{L}_1, \mathsf{L}_2$ can be spacetime translations. We assume the lattice model still has a finite period at both time and space directions, meaning that there exist $\alpha_1, \beta_1, \alpha_2, \beta_2 \in \mathbb{Z}$ such that $\mathsf{L}_x = \mathsf{L}_1^{\alpha_1}\mathsf{L}_2^{\beta_1}, \mathsf{L}_T = \mathsf{L}_1^{\alpha_2}\mathsf{L}_2^{\beta_2}$. By computing $\mathsf{L}_x\mathsf{L}_T\mathsf{L}_x^{-1}\mathsf{L}_T^{-1}$, we find that

$$\mathsf{L}_x\mathsf{L}_T\mathsf{L}_x^{-1}\mathsf{L}_T^{-1} = \sigma^{\alpha_1\beta_2-\alpha_2\beta_1}, \tag{97}$$

which indicates the flux $\Phi'$ contained in every loop formed by $\mathsf{L}_x\mathsf{L}_T\mathsf{L}_x^{-1}\mathsf{L}_T^{-1}$. One can show that the area circled by $\mathsf{L}_x\mathsf{L}_T\mathsf{L}_x^{-1}\mathsf{L}_T^{-1}$ is exactly $\alpha_1\beta_2 - \alpha_2\beta_1$ times the area circled by $\mathsf{L}_1\mathsf{L}_2\mathsf{L}_1^{-1}\mathsf{L}_2^{-1}$. On the other hand, the flux configuration must satisfies $\mathsf{L}_1$ and $\mathsf{L}_2$ symmetry. Therefore, the flux contained in every loop of the form $\mathsf{L}_1\mathsf{L}_2\mathsf{L}_1^{-1}\mathsf{L}_2^{-1}$ is exactly $\Phi = \Phi'/|\alpha_1\beta_2 - \alpha_2\beta_1|$, and we have

$$\sigma = e^{i\Phi\cdot \mathrm{sgn}(\alpha_1\beta_2-\alpha_2\beta_1)}, \tag{98}$$

where $\mathrm{sgn}(x)$ is the sign of $x$. If the direction of the loop $\mathsf{L}_1\mathsf{L}_2\mathsf{L}_1^{-1}\mathsf{L}_2^{-1}$ is the same as that of $\mathsf{L}_x\mathsf{L}_T\mathsf{L}_x^{-1}\mathsf{L}_T^{-1}$, $\mathrm{sgn}(\alpha_1\beta_2 - \alpha_2\beta_1) = 1$, otherwise $\mathrm{sgn}(\alpha_1\beta_2 - \alpha_2\beta_1) = -1$.

### *ii. Cohomology invariants of rotations*

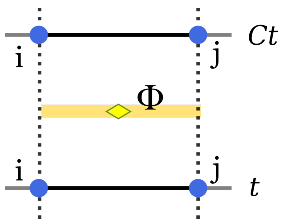


FIG. 15: Flux interpretation of the cohomology invariants of rotations. This lattice has $\mathsf{C}$ symmetry, and site $j = C(i)$.

For the rotations, the projective algebraic relation $\mathsf{C}^2 = \alpha$ requires that

$$\begin{aligned}\mathsf{C}^2 f(t)|i\rangle &= \mathsf{G}_c C \mathsf{G}_c C f(t)|i\rangle \\ &= \mathsf{G}_c(i)\mathsf{G}_c^{-1}(C(i))f(t)|i\rangle \qquad (99)\\ &= \alpha f(t)|i\rangle, \qquad (100)\end{aligned}$$

so the gauge transformation on sites satisfies

$$\mathsf{G}_c(i)\mathsf{G}_c^{-1}(C(i)) = \alpha. \tag{101}$$

Consider a lattice with $\mathsf{C}$ symmetry in Fig. 15, where site $j = C(i)$ and there can be some sites between $i$ and $j$. From Eq. (94), we get the constrain of the phases of hoppings:

$$e^{iA_{ij}(t)}e^{-iA_{ij}(Ct)} = \mathsf{G}_c^{-1}(i)\mathsf{G}_c(j) = (\mathsf{G}_c(i)\mathsf{G}_c^{-1}(C(i)))^{-1} = \alpha^{-1}, \tag{102}$$

The left hand side is $e^{-i\Phi}$, where $\Phi$ is the flux in the loop $(i,t) \to (j,t) \to (j,Ct) \to (i,Ct) \to (i,t)$, so we have the flux interpretation of cohomology invariants of rotations,

$$\alpha = e^{i\Phi}, \tag{103}$$

where $\Phi \in \pi\mathbb{Z}$ is the flux in every loop which is invariant under $\mathsf{C}$.

Note that, since $t$ can be very close to $Ct$, the loop can be infinitesimal, so the flux must concentrate on the time where the rotation center lies. For a $\pi$ flux, this indicates the hopping passing through the rotation center changes a minus sign after that time. When $t$ is the time at which the rotation center lies, i.e., $t = Ct$, we have $e^{iA_{ij}(t)}e^{-iA_{ij}(Ct)} = 1$, which seems to indicate the cohomology invariant $\alpha$ must be trivial. However, we can set $w_{ij}(t) = 0$ at this time, then the phases at this time can be arbitrary chosen, and we can choose $e^{iA_{ij}(t)}e^{-iA_{ij}(Ct)} = \alpha$ to preserve the projective symmetry.

*iii. Cohomology invariants between translations and reflections*

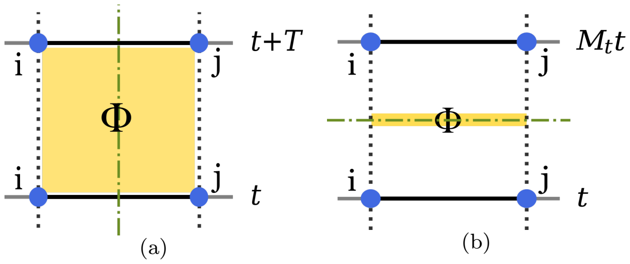


FIG. 16: (a) Flux interpretation of the cohomology invariants between $\mathsf{M}_x$ and $\mathsf{L}_T$. This lattice has $\mathsf{M}_x$ and $\mathsf{L}_T$ symmetry, and site $j = M_x(i)$. (b) Flux interpretation of the cohomology invariants between $\mathsf{M}_t$ and $\mathsf{L}_x$. This lattice has $\mathsf{M}_t$ and $\mathsf{L}_x$ symmetry, and site $j = L_x(i)$. Hoppings are taken to be real.

There are two kinds of cohomology invariants between translations and reflections, $\eta = [\mathsf{M}_x : \mathsf{L}_T]$ and $\overline{\eta} = [\mathsf{M}_t : \mathsf{L}_x]$. For the first type, the gauge transformations on sites satisfy the equation

$$\mathsf{G}_T(M_x^{-1}(i))\mathsf{G}_T^{-1}(i) = \eta. \tag{104}$$

Consider a lattice with $\mathsf{M}_x$ and $\mathsf{L}_T$ symmetry, as shown in Fig. 16(a), where site $j = M_x(i)$ and there can be some sites between $i$ and $j$. Taking $\mathsf{R} = \mathsf{L}_T$ in Eq. (94), we obtain

$$e^{iA_{ij}(t)}e^{-iA_{ij}(t+T)} = \mathsf{G}_T^{-1}(i)\mathsf{G}_T(j) = (\mathsf{G}_T(M^{-1}(j))\mathsf{G}_T^{-1}(j))^{-1} = \eta^{-1}. \tag{105}$$

Thus we have a flux interpretation of the cohomology invariant $\eta$ as

$$\eta = e^{i\Phi}, \tag{106}$$

where $\Phi \in \pi\mathbb{Z}$ is the flux in every loop formed by $\mathsf{M}_x\mathsf{L}_T\mathsf{M}_x^{-1}\mathsf{L}_T^{-1}$.

For the cohomology invariants $\overline{\eta} = [\mathsf{M}_t, \mathsf{L}_x]$, the gauge transformations on sites satisfy the equation

$$\mathsf{G}_m(i)\mathsf{G}_m^{-1}(L_x^{-1}(i)) = \overline{\eta}. \tag{107}$$

Consider a lattice with $\mathsf{M}_t$ and $\mathsf{L}_x$ symmetry, as shown in Fig. 16(b), where site $j = L_x(i)$. Takiing $\mathsf{R} = \mathsf{M}_t$ in Eq. (94), we have

$$e^{iA_{ij}(t)}e^{iA_{ij}(M_t t)} = \mathsf{G}_m(i)\mathsf{G}_m^{-1}(j) = \overline{\eta}^{-1}. \tag{108}$$

If we take all hoppings to be real such that $e^{A_{ij}(t)} = e^{-iA_{ij}(t)}$, then we have

$$\overline{\eta} = e^{i\Phi}, \tag{109}$$

where $\Phi \in \pi\mathbb{Z}$ is the flux in every loop formed by $\mathsf{M}_t\mathsf{L}_x\mathsf{M}_t^{-1}\mathsf{L}_x^{-1}$. Since the the loop can be infinitesimal, the flux must concentrate on the time reflection axis, and the hoppings that are static under $M_t$ should be set to 0 for $\overline{\eta} = -1$ case.

*iv. Cohomology invariants between translations and glide-reflections*

There are two types of cohomology invariants between translations and glide-reflections, $\tau = \mathsf{g}_t\mathsf{L}_T\mathsf{g}_t^{-1}\mathsf{L}_T$ and $\overline{\tau} = \mathsf{g}_x\mathsf{L}_x\mathsf{g}_x^{-1}\mathsf{L}_x$. For the first type, the gauge transformations on sites satisfy the equation

$$\mathsf{G}_T^{-1}(\mathsf{g}_t^{-1}(i))\mathsf{G}_T(i) = \tau. \tag{110}$$

Consider a lattice with $\mathsf{L}_T$ and $\mathsf{g}_t$ symmetry, as shown in Fig. 17(a), where site $j = g_t(i)$. Taking $\mathsf{R} = \mathsf{L}_T$ in Eq. (94), we obtain

$$e^{iA_{ij}(t)}e^{-iA_{ij}(t+T)} = \mathsf{G}_T^{-1}(i)\mathsf{G}_T(j) = \mathsf{G}_T^{-1}(\mathsf{g}_t^{-1}(j))\mathsf{G}_T(j) = \tau. \tag{111}$$

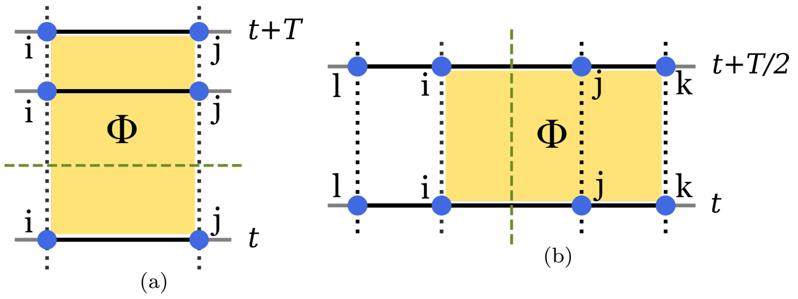


FIG. 17: (a) Flux interpretation of the cohomology invariants between $\mathsf{g}_x$ and $\mathsf{L}_T$. This lattice has $\mathsf{g}_t$ and $\mathsf{L}_T$ symmetry, and site $j = g_t(i)$. (b) Flux interpretation of the cohomology invariants between $\mathsf{g}_x$ and $\mathsf{L}_x$. This lattice has $\mathsf{g}_x$ and $\mathsf{L}_x$ symmetry, and site $j = g_x(i), k = L_x(i), l = L_x^{-1}(j)$.

The left-hand side is actually $e^{-i\Phi}$, where $\Phi$ is the flux in the loop formed by $\mathsf{g}_t\mathsf{L}_T\mathsf{g}_t^{-1}\mathsf{L}_T$ acting on site $i$. So we have the flux interpretation

$$\tau = e^{-i\Phi}, \tag{112}$$

where $\Phi$ is the flux in every loop formed by $\mathsf{g}_t\mathsf{L}_T\mathsf{g}_t^{-1}\mathsf{L}_T$.

It is interesting to note that

$$\mathsf{L}_x\mathsf{L}_T\mathsf{L}_x^{-1}\mathsf{L}_T^{-1} = \mathsf{g}_t^2\mathsf{L}_T\mathsf{g}_t^{-2}\mathsf{L}_T^{-1} = \tau^{-2}, \tag{113}$$

which means the flux in a loop formed by $\mathsf{L}_x\mathsf{L}_T\mathsf{L}_x^{-1}\mathsf{L}_T^{-1}$ is two times the flux in a loop formed by $\mathsf{g}_t\mathsf{L}_T\mathsf{g}_t^{-1}\mathsf{L}_T$.

For the cohomology invariant $\bar{\tau} = \mathsf{g}_x\mathsf{L}_x\mathsf{g}_x^{-1}\mathsf{L}_x$, the gauge transformations on sites satisfy the equation

$$\mathsf{G}_{g_x}(i)\mathsf{G}_x(g_x^{-1}(i))\mathsf{G}_{g_x}^{-1}(L_x(i))\mathsf{G}_x(L_x(i)) = \bar{\tau}. \tag{114}$$

Consider a lattice with $\mathsf{g}_x$ and $\mathsf{L}_x$ symmetry, as shown in Fig. 17(b), where site $j = g_x(i), k = L_x(i), l = L_x^{-1}(j)$. Taking $\mathsf{R} = \mathsf{g}_x$ and $\mathsf{R} = \mathsf{L}_x$ in Eq. (94) respectively, we have

$$e^{iA_{ij}(t)}e^{iA_{ij}(t+T/2)} = \mathsf{G}_{g_x}(i)\mathsf{G}_{g_x}^{-1}(j), \tag{115}$$

$$e^{iA_{li}(t)}e^{iA_{jk}(t+T/2)} = \mathsf{G}_{g_x}(j)\mathsf{G}_{g_x}^{-1}(k) \tag{116}$$

$$e^{-iA_{li}(t)}e^{iA_{jk}(t)} = \mathsf{G}_x(j)\mathsf{G}_x^{-1}(k), \tag{117}$$

then

$$e^{iA_{ij}(t)}e^{iA_{jk}(t)}e^{iA_{jk}(t+T/2)}e^{iA_{ij}(t+T/2)} = \mathsf{G}_{g_x}(i)\mathsf{G}_x(j)\mathsf{G}_{g_x}^{-1}(k)\mathsf{G}_x^{-1}(k). \tag{118}$$

If all hopping amplitudes are real, and the gauge transformations take values in $\mathbb{Z}_2$, then we have

$$\bar{\tau} = e^{i\Phi}, \tag{119}$$

where $\Phi \in \pi\mathbb{Z}$ is the flux in every loop formed by $\mathsf{g}_x\mathsf{L}_x\mathsf{g}_x^{-1}\mathsf{L}_x$.

### v. *Cohomology invariants of reflections*

There are two types of cohomology invariants of reflections, $\beta = \mathsf{M}_t^2$ and $\gamma = \mathsf{M}_x^2$.

The nontrivial cohomology invariant $\beta = -1$ can be realized by spinful systems. However, when there are two classes of time reversal axes corresponding to two cohomology invariants $\beta_1 = \mathsf{M}_t^2, \beta_2 = (\mathsf{L}_T\mathsf{M}_t)^2$ respectively, the cases $\beta_1 = -\beta_2$ cannot be realized. These cases occur for group $Pm_t$ and group $Pm_xm_t$. To address this issue, we realize $\beta = -1$ effectively by a two-layer model as shown in Fig. 18, where $\mathsf{M}_t$ is replaced by $\mathsf{R}\mathsf{M}_t$ ($\mathsf{R}$ is a horizontal two-fold spatial rotation). With this design, $\beta_1 = -\beta_2$ cases can be realized effectively by tuning hopping amplitudes.

The nontrivial cohomology invariant $\gamma = -1$ only appears in $\mathbb{Z}_2$-projective symmetry algebras. It cannot be realized in models with real hoppings. We can also realize it by a two-layer model as shown in Fig. 19, where $\mathsf{M}_x$ is replaced by a horizontal two-fold spatial rotation $\mathsf{R}$ effectively. $\gamma = -1$ corresponds to $\pi$ magnetic flux in the loops that are invariant under $R$.

In the following, we will focus on the realization of cohomology invariants $\sigma, \alpha, \eta, \bar{\eta}, \tau, \bar{\tau}$, and do not discuss the realization of $\beta$ and $\gamma$ anymore.

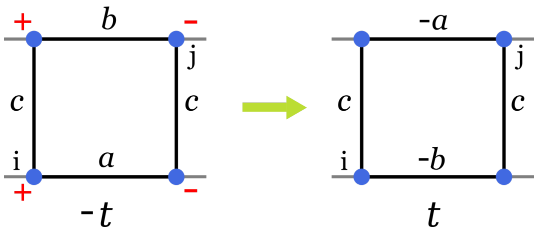


FIG. 18: Realization of $\beta = -1$ by a two-layer spacetime lattice. This figure shows the lattice at time $t$ and $-t$. We take all hoppings to be real. $\mathsf{M}_t$ is replaced by $\mathsf{RM}_t$ and site $j = RM_t(i)$, where $R$ is a horizental two-fold spatial rotation. The nontrivial projective symmetry algebra $(\mathsf{RM}_t)^2 = -1$ requires $\mathsf{G}(i)\mathsf{G}(j) = -1$. The red '+' and '-' symbols mark the gauge transformation $\mathsf{G}$.

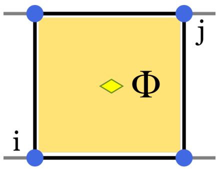


FIG. 19: Realization of $\gamma = -1$ by a two-layer spacetime lattice. This figure shows the lattice at one time. We take all hoppings to be real. $\mathsf{M}_x$ is replaced by $\mathsf{R}$ and site $j = R(i)$, where $R$ is a two-fold spatial rotation. When $\Phi = \pi$, we have $\mathsf{R}^2 = -1$.

## D. Lattice realization of projective symmetry algebras of (1,1)D spacetime crystalline groups

For all figures in this section, the letters near the hoppings label the strengths of the hoppings, while the phases of hoppings are determined by the fluxes.

### 1. P1

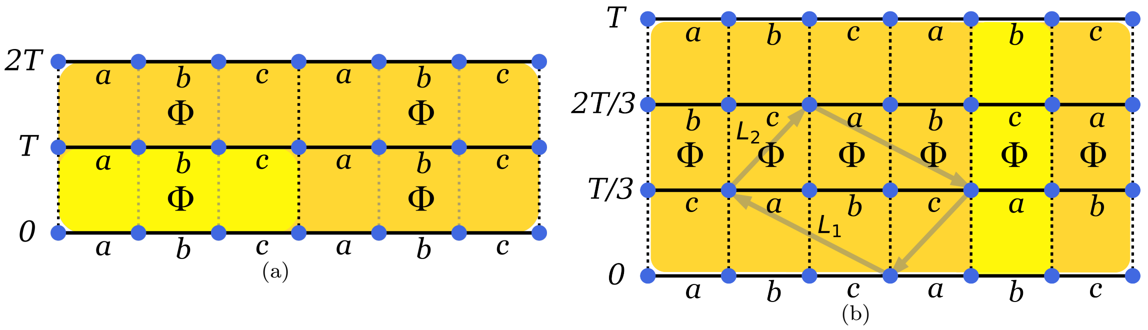


FIG. 20: Spacetime tight binding model with projective $P1$ symmetry. The bright area contains flux $\Phi$ such that every spacetime unit translation plaquette contains flux $\Phi$, which corresponds to the cohomology invariant $\sigma$. (a) Projective $P1$ symmetry model with spatial and time translation symmetry. (b) Projective $P1$ symmetry model with general spacetime translation symmetry.

Projective symmetry algebras of $P1$ have one independent cohomology invariant $\sigma = \mathsf{L}_1\mathsf{L}_2\mathsf{L}_1^{-1}\mathsf{L}_2^{-1}$. For $U(1)$ case, $\sigma \in U(1)$, and for $\mathbb{Z}_2$ case, $\sigma \in \mathbb{Z}_2$. According to what we analyzed in last section, we only need to add flux $\Phi$ to each unit translation plaquette to realize it, as shown in Fig. 20. The relation between the cohomology invariant and flux is

$$\sigma = e^{i\Phi}. \tag{120}$$

### 2. P2

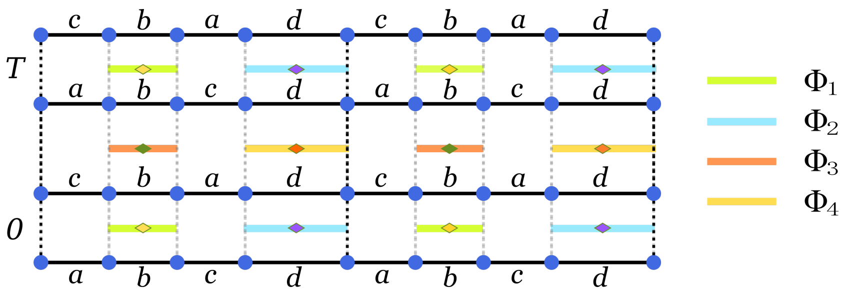


FIG. 21: Spacetime tight binding model with projective $P2$ symmetry. Flux $\Phi_1, \Phi_2, \Phi_3, \Phi_4$ corresponds to cohomology invariant $\alpha_1, \alpha_2, \alpha_3, \alpha_4$ respectively. The line shape of the flux means the flux concentrates on a line.

For spacetime group $P2$, there are four independent cohomology invariants $\alpha_1, \alpha_2, \alpha_3, \alpha_4 \in \mathbb{Z}_2$ of rotations for both $U(1)$ and $\mathbb{Z}_2$ cases. We can add $\Phi_1, \Phi_2, \Phi_3, \Phi_4 \in \pi\mathbb{Z}$ into every corresponding loops so that

$$\alpha_i = e^{i\Phi_i}, \quad i = 1, 2, 3, 4. \tag{121}$$

One example is shown in Fig. 21.

### 3. $\mathrm{Pm_x}$

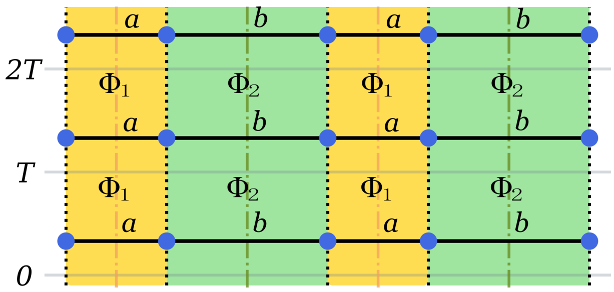


FIG. 22: Spacetime tight binding model with projective $Pm_x$ symmetry. Flux $\Phi_1, \Phi_2$ corresponds to cohomology invariant $\eta_1, \eta_2$ respectively. The hoppings should be real to keep $\mathsf{M}_x$ symmetry.

For $U(1)$-projective symmetry algebras of spacetime group $Pm_x$, there are two independent cohomology invariants $\eta_1, \eta_2 \in \mathbb{Z}_2$. We can realize them by adding $\Phi_1, \Phi_2 \in \pi\mathbb{Z}$ into every loop formed by $\mathsf{M}_x\mathsf{L}_T\mathsf{M}_x^{-1}\mathsf{L}_T^{-1}$ and $\mathsf{L}_x\mathsf{M}_x\mathsf{L}_T(\mathsf{L}_x\mathsf{M}_x)^{-1}\mathsf{L}_T^{-1}$ respectively. One example is shown in Fig. 22. The relations between flux configuration and cohomology invariants are

$$\eta_i = e^{i\Phi_i}, \qquad i = 1, 2. \tag{122}$$

Here we note that the adding of $\Phi_i$ should not break the spatial reflection symmetry.

For $\mathbb{Z}_2$-projective symmetry algebras of spacetime group $Pm_x$, there are four independent cohomology invariants $\eta_1, \eta_2, \gamma_1, \gamma_2 \in \mathbb{Z}_2$. $\eta_1, \eta_2$ can be also realized in the same way as $U(1)$ case.

#### 4. $\mathrm{Pm_t}$

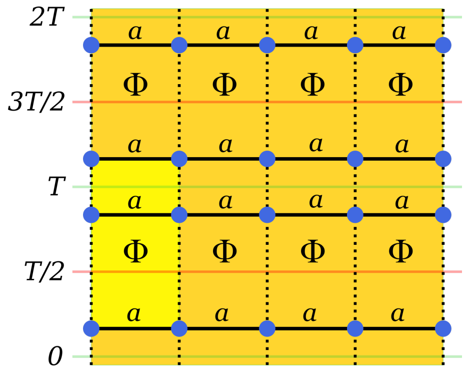


FIG. 23: Spacetime tight binding model with $U(1)$-projective $Pm_t$ symmetry. The bright area is one spacetime unit translation plaquette. In every spacetime unit translation plaquette, there is flux $\Phi$, which corresponds to the cohomology invariant $\sigma$.

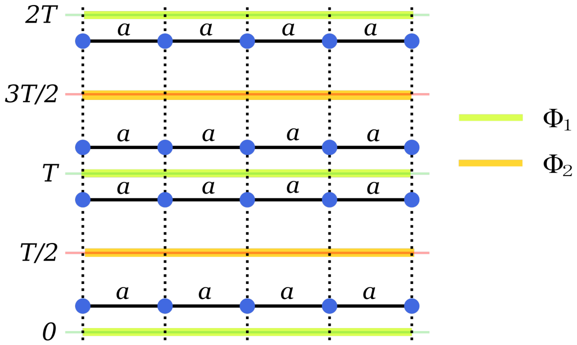


FIG. 24: Spacetime tight binding model with $\mathbb{Z}_2$-projective $Pm_t$ symmetry. There is $\Phi_1(\Phi_2)$ flux at $nT(nT+T/2)$ for every hopping. Flux $\Phi_1, \Phi_2$ corresponds to cohomology invariant $\overline{\eta}_1, \overline{\eta}_2$ respectively. In this model, all hoppings are real.

For $U(1)$-projective symmetry algebras of spacetime group $Pm_t$, there are three independent cohomology invariants $\sigma, \beta_1, \beta_2$. $\sigma \in U(1)$ can be realized by adding $\Phi$ flux into every loop formed by $\mathsf{L}_x \mathsf{L}_T \mathsf{L}_x^{-1} \mathsf{L}_T^{-1}$, as shown in Fig. 23. The relation between flux configuration and cohomology invariant $\sigma$ is

$$\sigma = e^{i\Phi}. \tag{123}$$

For $\mathbb{Z}_2$-projective symmetry algebras of spacetime group $Pm_t$, there are four independent cohomology invariants $\overline{\eta}_1, \overline{\eta}_2, \beta_1, \beta_2 \in \mathbb{Z}_2$. $\overline{\eta}_1, \overline{\eta}_2$ can be realized by adding flux $\Phi_1, \Phi_2 \in \pi\mathbb{Z}$ into every loop formed by $\mathsf{M}_t \mathsf{L}_x \mathsf{M}_t^{-1} \mathsf{L}_x^{-1}$ and $\mathsf{L}_T \mathsf{M}_t \mathsf{L}_x (\mathsf{L}_T \mathsf{M}_t)^{-1} \mathsf{L}_x^{-1}$ respectively, as shown in Fig. 24. The relations between flux configuration and cohomology invariants are

$$\overline{\eta}_i = e^{i\Phi_i}, \quad i = 1, 2. \tag{124}$$

### 5. $\mathrm{Pm_xm_t}$

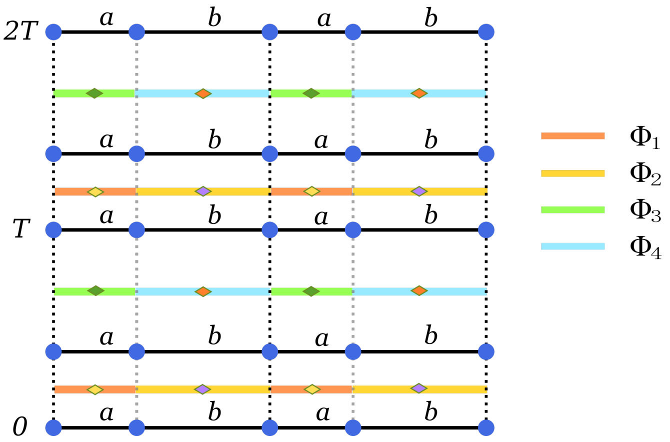


FIG. 25: Spacetime tight binding model with projective $Pm_xm_t$ symmetry. Flux $\Phi_1, \Phi_2, \Phi_3, \Phi_4$ corresponds to cohomology invariant $\alpha_1, \alpha_2, \alpha_3, \alpha_4$ respectively.

For $U(1)$-projective symmetry algebras of spacetime group $Pm_xm_t$, there are six independent cohomology invariants $\alpha_1, \alpha_2, \alpha_3, \alpha_4, \beta_1, \beta_2 \in \mathbb{Z}_2$. $\alpha_1, \alpha_2, \alpha_3, \alpha_4$ can be realized by adding $\Phi_1, \Phi_2, \Phi_3, \Phi_4 \in \pi\mathbb{Z}$ flux into every loop which is invariant under $\mathsf{M}_x\mathsf{M}_t, \mathsf{L}_x\mathsf{M}_x\mathsf{M}_t, \mathsf{L}_T\mathsf{M}_x\mathsf{M}_t, \mathsf{L}_x\mathsf{L}_T\mathsf{M}_x\mathsf{M}_t$ respectively, as shown in Fig. 25. The relations between flux configuration and cohomology invariants are

$$\alpha_i = e^{i\Phi_i}, \qquad i = 1, 2, 3, 4. \tag{125}$$

For $\mathbb{Z}_2$-projective symmetry algebras of spacetime group $Pm_xm_t$, there are eight independent cohomology invariants $\alpha_1, \alpha_2, \alpha_3, \alpha_4, \beta_1, \beta_2, \gamma_1, \gamma_2 \in \mathbb{Z}_2$. $\alpha_1, \alpha_2, \alpha_3, \alpha_4$ can be realized in the same way as $U(1)$ case.

### 6. $\mathrm{Pg_x}$

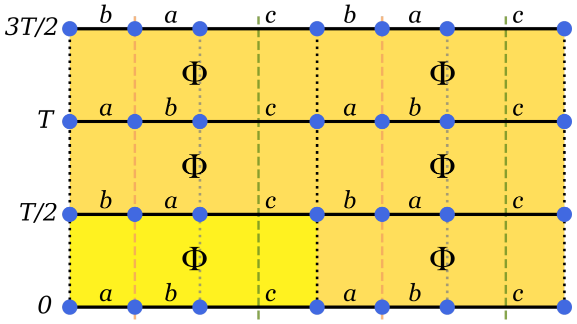


FIG. 26: Spacetime tight binding model with $\mathbb{Z}_2$-projective $Pg_x$ symmetry. The bright area is circled by one loop formed by $\mathsf{g}_x\mathsf{L}_x\mathsf{g}_x^{-1}\mathsf{L}_x$. In every such loop, there is flux $\Phi$, which corresponds to the cohomology invariant $\overline{\tau}$. All hoppings in this model is real.

For $U(1)$-projective symmetry algebras of spacetime group $Pg_x$, there is no nontrivial cohomology invariant.

For $\mathbb{Z}_2$-projective symmetry algebras of spacetime group $Pg_x$, there is one independent cohomology invariant $\overline{\tau} \in \mathbb{Z}_2$, which can be realized by adding $\Phi \in \pi\mathbb{Z}$ flux into everly loop formed by $\mathsf{g}_x\mathsf{L}_x\mathsf{g}_x^{-1}\mathsf{L}_x$, as shown in Fig. 26. We have the relation

$$\overline{\tau} = e^{i\Phi}. \tag{126}$$

### 7. $\mathrm{Pg_t}$

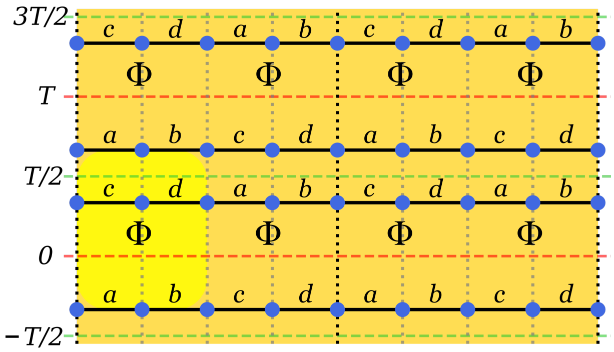


FIG. 27: Spacetime tight binding model with projective $Pg_t$ symmetry. The bright area is circled by one loop formed by $\mathsf{g}_t\mathsf{L}_T\mathsf{g}_t^{-1}\mathsf{L}_T$. In every such loop, there is flux $\Phi$, which corresponds to the cohomology invariant $\tau$.

projective symmetry algebras of $Pg_t$ have one independent cohomology invariant $\tau$. For $U(1)$ case, $\tau \in U(1)$, and for $\mathbb{Z}_2$ case, $\tau \in \mathbb{Z}_2$. $\tau$ can be realized by adding flux $\Phi$ into every loop formed by $\mathsf{g}_t\mathsf{L}_T\mathsf{g}_t^{-1}\mathsf{L}_T$, as shown in Fig. 27. The relation between flux configuration and cohomology invariant is

$$\tau = e^{-i\Phi}. \tag{127}$$

### 8. $\mathrm{Pg_xg_t}$

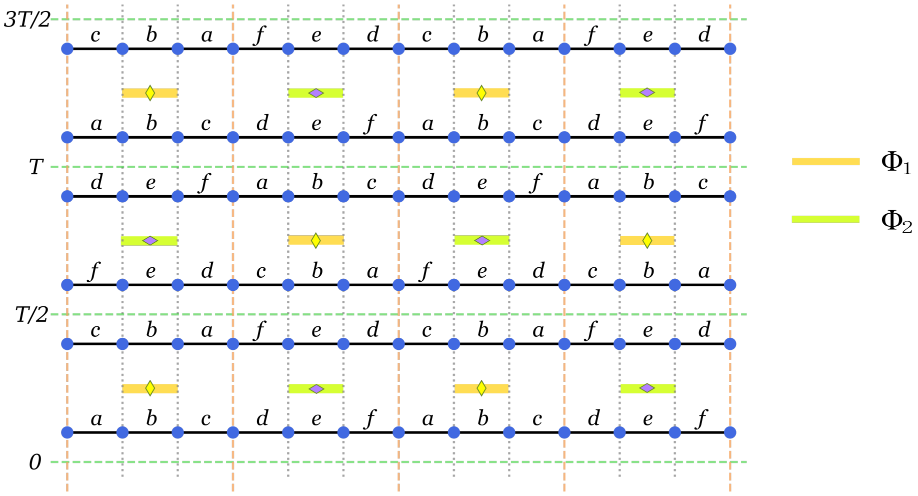


FIG. 28: Spacetime tight binding model with projective $Pg_xg_t$ symmetry. Flux $\Phi_1, \Phi_2$ corresponds to cohomology invariant $\alpha_1, \alpha_2$ respectively.

For both $U(1)$ and $\mathbb{Z}_2$ projective symmetry algebras of $Pg_xg_t$, there are two independent cohomology invariants $\alpha_1, \alpha_2 \in \mathbb{Z}_2$, which can be realized by adding $\Phi_1, \Phi_2 \in \pi\mathbb{Z}$ flux into every loop which is invariant under rotation $\mathsf{g}_x\mathsf{g}_t, \mathsf{g}_x\mathsf{g}_t^{-1}$ respectively. One example is shown in Fig. 28. The relations between flux configuration and cohomology invariants are

$$\alpha_i = \Phi_i, \quad i = 1, 2. \tag{128}$$

**9.** $\mathrm{Pm_xg_t}$

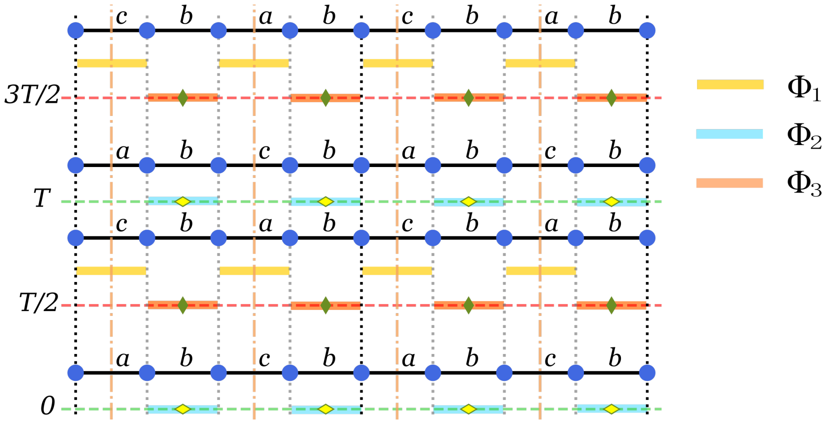


FIG. 29: Spacetime tight binding model with projective $Pm_xg_t$ symmetry. Flux $\Phi_1, \Phi_2, \Phi_3$ corresponds to cohomology invariant $\eta, \alpha_1, \alpha_2$ respectively.

For $U(1)$-projective symmetry algebras of spacetime group $Pm_xg_t$, there are three independent cohomology invariants $\eta, \alpha_1, \alpha_2 \in \mathbb{Z}_2$. $\eta$ can be realized by adding $\Phi_1 \in \pi\mathbb{Z}$ flux into every loop formed by $\mathsf{M}_x\mathsf{L}_T\mathsf{M}_x^{-1}\mathsf{L}_T^{-1}$. $\alpha_1, \alpha_2$ can be realized by adding $\Phi_2, \Phi_3 \in \pi\mathbb{Z}$ flux into every loop which is invariant under $\mathsf{M}_x\mathsf{g}_t$ and $\mathsf{L}_T\mathsf{M}_x\mathsf{g}_t$ respectively. One example is shown in Fig. 29. The relations between flux configuration and cohomology invariants are

$$\eta = e^{i\Phi_1}, \tag{129}$$

$$\alpha_1 = e^{i\Phi_2}, \tag{130}$$

$$\alpha_2 = e^{i\Phi_3}. \tag{131}$$

For $\mathbb{Z}_2$-projective symmetry algebras of spacetime group $Pm_xg_t$, there are four independent cohomology invariants $\eta, \alpha_1, \alpha_2, \gamma \in \mathbb{Z}_2$. $\eta, \alpha_1, \alpha_2$ can be realized in the same way as $U(1)$ case.

**10.** $\mathrm{Pm_tg_x}$

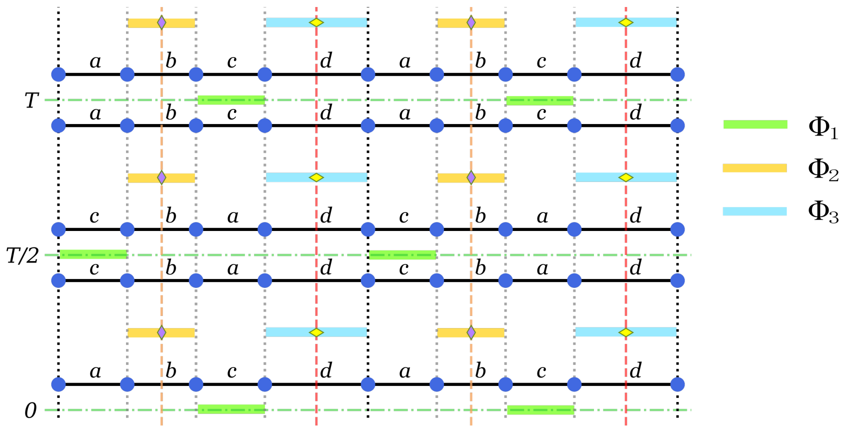


FIG. 30: Spacetime tight binding model with projective $Pm_tg_x$ symmetry. Flux $\Phi_1, \Phi_2$ corresponds to cohomology invariant $\alpha_1, \alpha_2$ respectively. For $\mathbb{Z}_2$-projective symmetry algebras, hoppings are taken to be all real and $\Phi_3$ corresponds to cohomology invariant $\overline{\eta}$.

For $U(1)$-projective symmetry algebras of spacetime group $Pm_tg_x$, there are three independent cohomology invariants $\alpha_1, \alpha_2, \beta \in \mathbb{Z}_2$. $\alpha_1, \alpha_2$ can be realized by adding $\Phi_1, \Phi_2 \in \pi\mathbb{Z}$ flux into every loop which is invariant under $\mathsf{M}_t\mathsf{g}_x$ and $\mathsf{L}_x\mathsf{M}_t\mathsf{g}_x$ respectively.

For $\mathbb{Z}_2$-projective symmetry algebras of spacetime group $Pm_tg_x$, there are four independent cohomology invariants $\overline{\eta}, \alpha_1, \alpha_2, \beta \in \mathbb{Z}_2$. $\alpha_1, \alpha_2$ can be realized in the way as $U(1)$ case. $\overline{\eta}$ can be realized by adding flux $\Phi_3$ into every loop formed by $\mathsf{M}_t\mathsf{L}_x\mathsf{M}_t^{-1}\mathsf{L}_x^{-1}$. If $\overline{\eta} = -1$, all hoppings should be real.

One example is shown in Fig. 30. The relations between flux configuration and cohomology invariants are

$$\alpha_1 = e^{i\Phi_1}, \tag{132}$$
$$\alpha_2 = e^{i\Phi_2}, \tag{133}$$
$$\overline{\eta} = e^{i\Phi_3}. \tag{134}$$
$$\tag{135}$$

### 11. $\mathrm{Cm_x}$

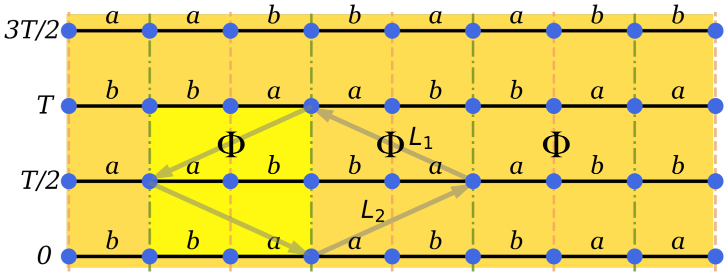


FIG. 31: Spacetime tight binding model with projective $Cm_x$ symmetry. One loop formed by $\mathsf{L}_1\mathsf{L}_2\mathsf{L}_1^{-1}\mathsf{L}_2^{-1}$ is marked by arrows. The bright area contains $\Phi$ flux, which corresponds to the cohomology invariant $\sigma$. $\Phi$ should not break the $\mathsf{M}_x$ symmetry.

For $U(1)$-projective symmetry algebras of spacetime group $Cm_x$, there are one independent cohomology invariant $\sigma \in \mathbb{Z}_2$, which can be realized by adding $\Phi \in \pi\mathbb{Z}$ flux into every loop formed by $\mathsf{L}_1\mathsf{L}_2\mathsf{L}_1^{-1}\mathsf{L}_2^{-1}$. This can be done by adding $2\Phi$ flux into every loop formed by $\mathsf{L}_x\mathsf{L}_T\mathsf{L}_x^{-1}\mathsf{L}_T^{-1}$ and making the flux configuration satisfy $Cm_x$ symmetry. One example is shown in Fig. 31. The relation between flux configuration and cohomology invariant is

$$\sigma = e^{i\Phi}. \tag{136}$$

Here we note that the adding of $\Phi_i$ should not break the spatial reflection symmetry.

For $\mathbb{Z}_2$-projective symmetry algebras of spacetime group $Cm_x$, there are two independent cohomology invariants $\sigma, \gamma \in \mathbb{Z}_2$. $\sigma$ can also be realized in the same way as $U(1)$ case.

### 12. $\mathrm{Cm_t}$

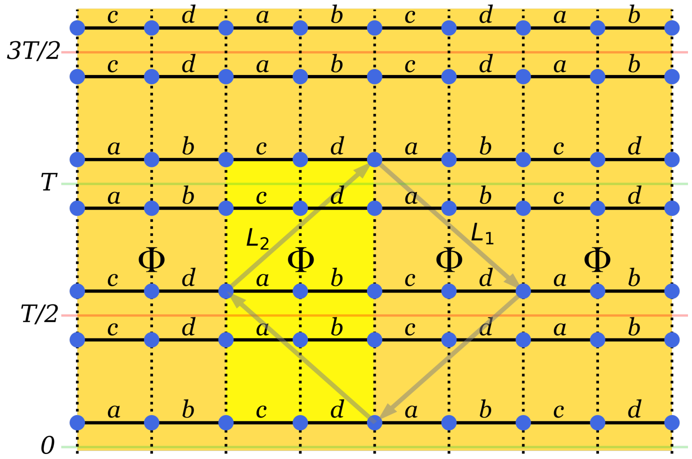


FIG. 32: Spacetime tight binding model with projective $Cm_t$ symmetry. One loop formed by $\mathsf{L}_1\mathsf{L}_2\mathsf{L}_1^{-1}\mathsf{L}_2^{-1}$ is marked by arrows. The bright area contains $\Phi$ flux, which corresponds to the cohomology invariant $\sigma$.

For $U(1)$-projective symmetry algebras of spacetime group $Cm_t$, there are two independent cohomology invariants $\sigma \in U(1), \beta \in \mathbb{Z}_2$. $\sigma$ can be realized by adding $\Phi$ flux into every loop formed by $\mathsf{L}_1\mathsf{L}_2\mathsf{L}_1^{-1}\mathsf{L}_2^{-1}$. This can be done by adding $2\Phi$ flux into every loop formed by $\mathsf{L}_x\mathsf{L}_T\mathsf{L}_x^{-1}\mathsf{L}_T^{-1}$ and making the flux configuration satisfy $Cm_t$ symmetry. One example is shown in Fig. 32. The relation between flux configuration and cohomology invariant is

$$\sigma = e^{\pm i\Phi}, \tag{137}$$

where the sign is positive if $\mathsf{L}_1\mathsf{L}_2\mathsf{L}_1^{-1}\mathsf{L}_2^{-1}$ has the same direction with $\mathsf{L}_x\mathsf{L}_T\mathsf{L}_x^{-1}\mathsf{L}_T^{-1}$, otherwise the sign is negative.

For $\mathbb{Z}_2$-projective symmetry algebras of spacetime group $Cm_t$, there are two independent cohomology invariants $\sigma, \gamma \in \mathbb{Z}_2$. $\sigma$ can also be realized in the same way as $U(1)$ case.

### 13. $\mathrm{Cm_xm_t}$

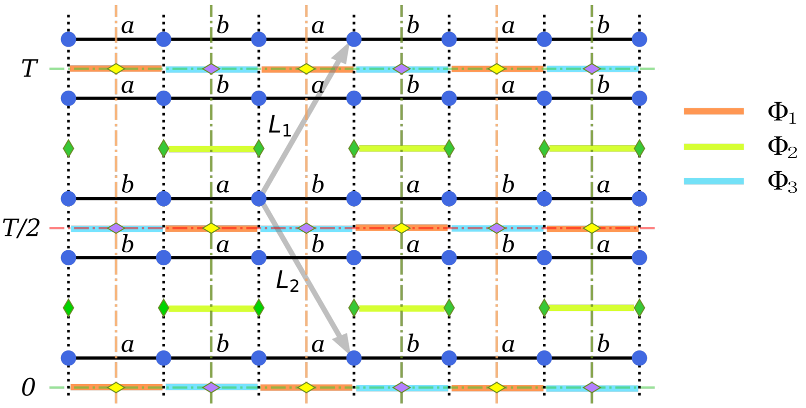


FIG. 33: Spacetime tight binding model with projective $Cm_xm_t$ symmetry. Flux $\Phi_1, \Phi_2, \Phi_3$ corresponds to cohomology invariant $\alpha_1, \alpha_2, \alpha_3$ respectively.

For $U(1)$-projective symmetry algebras of spacetime group $Cm_xm_t$, there are four independent cohomology invariants $\alpha_1, \alpha_2, \alpha_3, \beta \in \mathbb{Z}_2$. $\alpha_1, \alpha_2, \alpha_3$ can be realized by adding $\Phi_1, \Phi_2, \Phi_3 \in \pi\mathbb{Z}$ flux into every loop which is invariant under rotation $\mathsf{M}_x\mathsf{M}_t$, $\mathsf{L}_1\mathsf{M}_x\mathsf{M}_t$ and $\mathsf{L}_1\mathsf{M}_x\mathsf{L}_1^{-1}\mathsf{M}_t$ respectively. One example is shown in Fig. 33. The relations between

flux configuration and cohomology invariants are

$$\alpha_i = e^{i\Phi_i}, \quad i = 1, 2, 3. \tag{138}$$

For $\mathbb{Z}_2$-projective symmetry algebras of spacetime group $Cm_x m_t$, there are five independent cohomology invariants $\alpha_1, \alpha_2, \alpha_3, \beta, \gamma \in \mathbb{Z}_2$. $\alpha_1, \alpha_2, \alpha_3$ can also be realized in the same way as $U(1)$ case.

## E. Other details

### 1. Proof of the electric Floquet-Bloch theorem

First, we review the proof of the ordinary Floquet-Bloch theorem. This theorem states that for a periodic driving system $H(\mathbf{r}, t)$, where $H(\mathbf{r} + \mathbf{a}_i, t) = H(\mathbf{r}, t + T) = H(\mathbf{r}, t)$, the solutions of the time-dependent equation $i\partial_t \psi(\mathbf{r}, t) = H(\mathbf{r}, t)\psi(\mathbf{r}, t)$ can be linearly composed by the Floquet-Bloch states

$$\begin{aligned} &\psi_{k,n}(\mathbf{r}, t) = e^{i\mathbf{k}\cdot\mathbf{r} - i\epsilon_n(\mathbf{k})t} u_{k,n}(\mathbf{r}, t), \\ &u_{k,n}(\mathbf{r} + \mathbf{a}_i, t) = u_{k,n}(\mathbf{r}, t), \\ &u_{k,n}(\mathbf{r}, t + T) = u_{k,n}(\mathbf{r}, t). \end{aligned} \tag{139}$$

For simplicity, we only review the proof of this theorem for 1+1D, and the generalization to 3+1D is straightforward. In 1+1D, there are two translation operators $L_x, L_T$, defined as $L_x f(x, t) = f(x + a, t)$, $L_T f(x, t) = f(x, t + T)$, respectively. The spacetime translation group $G$ is generated by $L_x$ and $L_T$, and is an abelian group since $L_x$ commutes with $L_T$. We define the operator

$$\mathcal{H}(x, t) = H(x, t) - i\partial_t. \tag{140}$$

Then, the solutions satisfy $\mathcal{H}(x, t)\psi(x, t) = 0$. All solutions form a solution space $V$.

Because $L_x$ and $L_T$ both commute with $\mathcal{H}(x, t)$, every group element $g \in G$ also commutes with $\mathcal{H}(x, t)$. This implies that the solution space $V$ is a representation of $G$, which can be decomposed into a direct sum of irreducible representations of $G$. Since $G$ is abelian, its irreducible representations are one dimensional. These irreducible representations are labelled by $(k, \epsilon)$, with character $\chi_{k,\epsilon}((L_x)^n (L_T)^m) = e^{ikna - i\epsilon mT}$, $m, n \in \mathbb{Z}$. The range of $(k, \epsilon)$ is $k \in [0, 2\pi/a)$, $\epsilon \in [0, 2\pi/T)$. If a solution $\psi(x, t)$ belongs to an irreducible representation labelled by $(k, \epsilon)$, it satisfies

$$\begin{aligned} &L_x \psi(x, t) = e^{ika} \psi(x, t), \\ &L_T \psi(x, t) = e^{-i\epsilon T} \psi(x, t). \end{aligned} \tag{141}$$

We can rewrite these conditions as

$$\begin{aligned} &\psi(x, t) = e^{ikx - i\epsilon t} u(x, t), \\ &u(x + a, t) = u(x, t), \\ &u(x, t + T) = u(x, t). \end{aligned} \tag{142}$$

Plug this ansatz into $\mathcal{H}(x, t)\psi(x, t) = 0$, we have

$$(H(k, t) - i\partial_t) u(x, t) = \epsilon u(x, t), \tag{143}$$

where $H(k, t) = e^{-ika} H(x, t) e^{ika}$. By solving this equation, we can obtain a set of eigenvalues $\epsilon_n(k)$ and corresponding eigenstates $u_{k,n}(x, t)$. So we can label each state with $(k, n)$, i.e., $\psi_{k,n}(x, t) = e^{ikx - i\epsilon_n(k)t} u_{k,n}(x, t)$. A general solution is a linear combination of $\psi_{k,n}(x, t)$. Thus, we have complete the proof of the Floquet-Bloch theorem.

Now, let us prove the Floquet-Bloch theorem in a uniform electric field, which we call electric Floquet-Bloch theorem. We also only concern the 1+1D case. The Hamiltonian for a periodic driving system in a uniform electric field $E_x = E$ can be written as

$$H(x, t) = -\frac{1}{2m}(\partial_x - iA_x(t))^2 + U(x, t). \tag{144}$$

Here we choose the gauge $A_0 = 0$, $A_x(t) = -Et$. Now, although $U(x, t)$ is periodic, i.e, $U(x + a, t) = U(x, t + T) = U(x, t)$, $H(x, t)$ is not periodic in time, i.e., $H(t + T) \neq H(t)$. However, we observe that $H(x, t + T)$ only differs from

$H(x,t)$ by a gauge transformation $A_x \to A_x + \partial_x \chi(x),\ \chi(x) = ETx$. This gauge transformation can be equivalently defined as

$$H(x,t) \to G_T H(x,t) G_T^{-1} = e^{i\chi(x)} H(x,t) e^{-i\chi(x)}, \tag{145}$$

where $G_T = e^{i\chi(x)}$. So now we can define a proper time translation operator $\mathsf{L}_T = G_T L_T$ which commutes with $H(x,t)$, i.e., $\mathsf{L}_T H(x,t) \mathsf{L}_T^{-1} = H(x,t)$. Moreover, one can verify that the two proper translation operators $\mathsf{L}_T$ and $L_x$ satisfy the following equation:

$$L_x \mathsf{L}_T L_x^{-1} \mathsf{L}_T^{-1} = e^{iEaT} = e^{i\Phi_E}, \tag{146}$$

where $\Phi_E = EaT$ is the electric flux in every spacetime unit cell. We assume it to be a rational, $\Phi_E = p\Phi_0/q = 2\pi p/q$.

To find the constrain of the translation symmetry on the wavefunction, we need to find commutative operators that commute with the Hamiltonian. Here, we can take $L_x, (\mathsf{L}_T)^q$ as two generators. They generate an abelian spacetime translation group $G$. Every group element $g \in G$ commutes with $\mathcal{H}(x,t)$. Therefore, the solution space $V$ is a representation of $G$. The one dimensional irreducible representations of $G$ are also labelled by $(k,\epsilon)$, but now the range of $(k,\epsilon)$ is $k \in [0, 2\pi/a),\ \epsilon \in [0, 2\pi/qT)$. If a solution $\psi(x,t)$ belongs to a representation labelled by $(k,\epsilon)$, it satisfies

$$\begin{aligned} L_x \psi(x,t) &= e^{ika}\psi(x,t), \\ (\mathsf{L}_T)^q \psi(x,t) &= e^{-i\epsilon q T}\psi(x,t), \end{aligned} \tag{147}$$

which can be rewritten as

$$\begin{aligned} \psi(x+a,t) &= e^{ika}\psi(x,t), \\ \psi(x,t+qT) &= e^{-iETx} e^{-i\epsilon qT}\psi(x,t) = e^{-i2\pi p x/a} e^{-i\epsilon qT}\psi(x,t). \end{aligned} \tag{148}$$

We can rewrite it as

$$\begin{aligned} \psi(x,t) &= e^{ikx - i\epsilon t} u(x,t), \\ u(x+a,t) &= u(x,t), \\ u(x,t+qT) &= e^{-i2\pi p x/a} u(x,t). \end{aligned} \tag{149}$$

Plug this ansatz into $\mathcal{H}(x,t)\psi(x,t) = 0$, we can obtain a set of eigenvalues $\epsilon_n(k)$ and eigenstates $u_{n,k}(x,t)$. Hence we can label a state with by $(k,n)$ and finally we derive the electric Floquet-Bloch theorem in the main text.

Since $[\mathcal{H}(x,t), \mathsf{L}_T]$=0, if $\psi_{k,n}(x,t)$ is a solution, $\psi'(x,t) = \mathsf{L}_T \psi_{k,n}(x,t) = e^{i\chi(x)}\psi_{k,n}(x,t+T)$ is also a solution with the same quasienergy $\epsilon_n(k)$ but momentum $k + 2\pi p/qa$. This can be seen by

$$\begin{aligned} (\mathsf{L}_T)^q \psi'(x,t) &= (\mathsf{L}_T)^q \mathsf{L}_T \psi_{k,n}(x,t) = \mathsf{L}_T (\mathsf{L}_T)^q \psi_{k,n}(x,t) = e^{-i\epsilon_n(k)qT} \mathsf{L}_T \psi_{k,n}(x,t) = e^{-i\epsilon_n(k)qT}\psi'(x,t), \\ L_x \psi'(x,t) &= L_x \mathsf{L}_T \psi_{k,n}(x,t) = e^{i\Phi_E} \mathsf{L}_T L_x \psi_{k,n}(x,t) = e^{i2\pi p/q} e^{ika} \mathsf{L}_T \psi_{k,n}(x,t) = e^{i(k+2\pi p/qa)a}\psi'(x,t). \end{aligned} \tag{150}$$

With this reason, $\mathsf{L}_T^m \psi_{k,n}(x,t),\ m = 0,1,2,...,q-1$ are $q$-fold degenerate Floquet-Bloch states, wherein $\mathsf{L}_T^m \psi_{k,n}(x,t)$ has momentum $k + 2\pi m p/qa$.

### 2. Kramers degeneracy protected by projective P2 symmetry

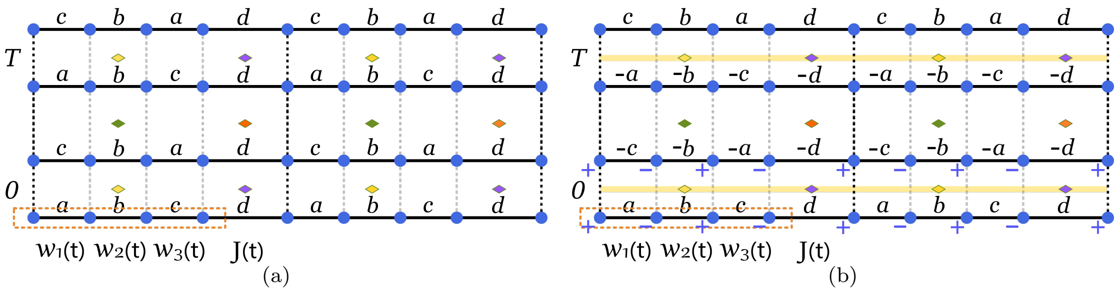


FIG. 34: (a) $P2$ spacetime tight binding model. (b) Projective $P2$ spacetime tight binding model with projective symmetry algebra $\mathsf{C}^2 = (L_x\mathsf{C})^2 = -1, (\mathsf{L}_T\mathsf{C})^2 = (\mathsf{L}_T L_x \mathsf{C})^2 = 1$. Hoppings acquire an extra minus sign after passing the highlight lines. On these lines, hoppings are taken to be 0. The blue '+' and '-' signs represent gauge transformation $G_C$.

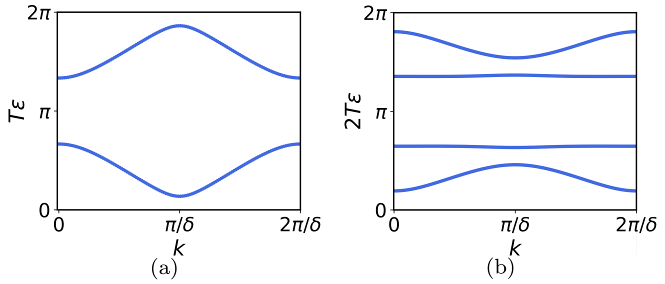


FIG. 35: (a) Quasibands of Floquet model with projective $P2$ symmetry in Fig. 34(b). Each band is two-fold degenerate. (b) Quasibands of Floquet model with ordinary $P2$ symmetry in Fig. 34(a). Parameters are given in Sec. E 4.

There can be Kramers degeneracy protected by projective $P2$ symmetry. Consider the lattice model with $P2$ symmetry in Fig. 34(a), whose Hamiltonian in momentum space is

$$H(k,t) = \begin{bmatrix} 0 & w_1(t) & 0 & J(t)e^{-ik\delta} \\ w_1(t) & 0 & w_2(t) & 0 \\ 0 & w_2(t) & 0 & w_3(t) \\ J(t)e^{ik\delta} & 0 & w_3(t) & 0 \end{bmatrix}, \tag{151}$$

where $w_1(t), w_2(t), w_3(t)$ are the inner cell hoppings and $J(t)$ is the intra cell hopping. All hoppings are $T$-periodic. The $P2$ symmetry require the hoppings satisfy $w_1(t) = w_3(-t),\ w_2(t) = w_2(-t),\ J(t) = J(-t)$. $\delta$ is the unit cell distance. The two-fold spacetime rotation operator $C$ in momentum space is represented as

$$C = M_x M_t = (\sigma_1 \otimes \sigma_1 \mathcal{I}_k)(\mathcal{I}_k \mathcal{K} \mathcal{I}_t) = \sigma_1 \otimes \sigma_1 \mathcal{K} \mathcal{I}_t, \tag{152}$$

where $\sigma_i$ are Pauli martices, $\mathcal{I}_k$ ($\mathcal{I}_t$) is the inversion of $k(t)$, and $\mathcal{K}$ is the complex conjugation. We have $C^2 = 1, (L_x C)^2 = 1, (L_T C)^2 = 1, (L_T L_x C)^2 = 1$.

Now consider the nontrivial projective symmetry algebra $\mathsf{C}^2 = -1,\ (\mathsf{L}_x\mathsf{C})^2 = -1, (\mathsf{L}_T\mathsf{C})^2 = 1, (\mathsf{L}_T\mathsf{L}_x\mathsf{C})^2 = 1$. This algebra can be realized by introducing a $\pi$ flux into every loop that is invariant under $\mathsf{C}$ or $(\mathsf{L}_x\mathsf{C})$, as illustrated in Fig. 34(b). Now the new Hamiltonian $H(k,t)$ has the same form of Eq. (151), but with hoppings satisfy $w_1(-t) = -w_3(t),\ w_2(-t) = -w_2(t),\ J(-t) = -J(t)$ and $w_i(t) = -w_i(t+T),\ i = 1,2,3,\ J(t) = -J(t+T)$. The proper rotation is $\mathsf{C} = G_C C$, where the gauge transformation $G_C$ in momentum space is represented as $G_C = \sigma_1 \otimes \sigma_3$. Therefore, $\mathsf{C}$ is represented as

$$\mathsf{C} = \sigma_1 \otimes i\sigma_2\ \mathcal{K}\mathcal{I}_t. \tag{153}$$

It can be verified that the new Hamiltonian satisfies $\mathsf{C}H(k,t)\mathsf{C}^{-1} = H(k,t)$, and we obtain the desired projective symmetry algebra $\mathsf{C}^2 = -1,\ (\mathsf{L}_x\mathsf{C})^2 = -1, (\mathsf{L}_T\mathsf{C})^2 = 1, (\mathsf{L}_T\mathsf{L}_x\mathsf{C})^2 = 1$.

From $\mathsf{C}H(k,t)\mathsf{C}^{-1} = H(k,t)$, we have

$$M_C H(k,t) M_C^{-1} = H^*(k,-t), \tag{154}$$

where $M_C = \sigma_1 \otimes i\sigma_2$. This relation implies the Kramers degeneracy of the quasibands at each $k$. Here is the proof. The quasienergies $\epsilon_n(k)$ are defined as eigenvalues of the evolution operator $U(k,2T) = \mathcal{T}\exp(-i\int_0^{2T} dt' H(k,t'))$, i.e., $U(k,2T)|\psi_{k,n}\rangle = e^{-i\epsilon_n(k)2T}|\psi_{k,n}\rangle$. From Eq. (154) we can prove

$$M_C U(k,2T) M_C^{-1} = U^{-1*}(k,2T). \tag{155}$$

If $|\psi\rangle$ is an eigenstate of $U(k,2T)$, then $M_C^{-1}\mathcal{K}|\psi\rangle$ is also an eigenstate. When $M_C M_C^* = -1$, which is the case for $M_C = \sigma_1 \otimes i\sigma_2$, $M_C^{-1}\mathcal{K}|\psi\rangle$ is linear independent with $|\psi\rangle$. So there is a two-fold Kramers degeneracy protected by the projective $P2$ symmetry. The quasibands for one set of parameters are shown in Fig. 35 (a), and we plot the quasibands of a model with ordinary $P2$ symmetry in Fig. 35 (b) for comparison.

### 3. Band crossing due to projective symmetry

Here, we consider a driven Su-Schrieffer-Heeger (SSH) model

$$H(t) = v(t)\sum_i c_{i,A}^\dagger c_{i,B} + w(t)\sum_i c_{i,B}^\dagger c_{i+1,A} + h.c. \tag{156}$$

where $v(t)$ and $w(t)$ are real. We require $H(t)$ to evolve adiabatically. We consider the case where the Hamiltonian exhibits projective time translation symmetry $H(t+T) = -H(t)$, which can be expressed as $GH(t+T)G^{-1} = H(t)$, with $G = \mathrm{diag}(+1,-1,+1,-1,...)$ in real space. Under this symmetry, the instantaneous bands of the system must cross at some time $t$. This is easy to see: In one period $T$, since $w(t+T) = -w(t), v(t+T) = -v(t)$, there exists a time $t_*$ at which $w(t_*) = v(t_*)$. Note that SSH model is gapless when $|w| = |v|$, which implies that the driven SSH model exhibits a band crossing at $t = t_*$.

### 4. Parameters of models

The parameters of the model in Fig. 2C in the main text are

$$w_1(t) = A\cos(\frac{\pi}{T_0}t), \quad t \in [0, 2T_0], \tag{157}$$

$$w_2(t) = \begin{cases} B - \frac{3B}{2T_0}t, \quad t \in [0, \frac{2T_0}{3}], \\ -\frac{3B}{T_0}(t - \frac{2T_0}{3}), \quad t \in [\frac{2T_0}{3}, T_0], \\ -(B - \frac{3B}{2T_0}(t - T_0)), \quad t \in [T_0, \frac{5T_0}{3}], \\ \frac{3B}{T_0}(t - \frac{5T_0}{3}), \quad t \in [\frac{5T_0}{3}, 2T_0], \end{cases} \tag{158}$$

$$J(t) = \begin{cases} C - \frac{3C}{T_0}t, \quad t \in [0, \frac{T_0}{3}], \\ -\frac{3C}{2T_0}(t - \frac{T_0}{3}), \quad t \in [\frac{T_0}{3}, T_0], \\ -(C - \frac{3C}{T_0}(t - T_0)), \quad t \in [T_0, \frac{4T_0}{3}], \\ \frac{3B}{2T_0}(t - \frac{4T_0}{3}), \quad t \in [\frac{4T_0}{3}, 2T_0]. \end{cases} \tag{159}$$

The original period is $T_0$, and when projectively represented, the period becomes $2T_0$. In Fig. 1(b) in the main text, we take $A = 3.5,\ B = 7,\ C = -6$.

For the model in Fig. 2D in the main text, the parameters are

When $t \in [0, T_0/2]$,

$$\begin{aligned} w_1(t) &= A\sin(\frac{\pi}{T_0}t), \\ w_2(t) &= B_0 + B\sin(\frac{\pi}{T_0}t), \\ w_3(t) &= \frac{2A}{T_0}t, \\ J(t) &= B_0 + \frac{2B}{T_0}t, \end{aligned} \tag{160}$$

when $t \in [T_0/2, T_0]$,

$$\begin{aligned} w_1(t) &= -\frac{2A}{T_0}(t - T_0), \\ w_2(t) &= B_0 - \frac{2B}{T}(t - T_0), \\ w_3(t) &= A\sin(\frac{\pi}{T_0}t), \\ J(t) &= B_0 + B\sin(\frac{\pi}{T_0}t), \end{aligned} \tag{161}$$

when $t \in [T_0, 3T_0/2]$,

$$\begin{aligned}
w_1(t) &= -A\sin(\frac{\pi}{T_0}(t-T_0)),\\
w_2(t) &= B_0 + B\sin(\frac{\pi}{T_0}(t-T_0)),\\
w_3(t) &= -\frac{2A}{T_0}(t-T_0),\\
J(t) &= B_0 + \frac{2B}{T_0}(t-T_0),
\end{aligned} \tag{162}$$

when $t \in [3T_0/2, 2T_0]$,

$$\begin{aligned}
w_1(t) &= \frac{2A}{T_0}(t-2T_0),\\
w_2(t) &= B_0 - \frac{2B}{T}(t-2T_0),\\
w_3(t) &= -A\sin(\frac{\pi}{T_0}(t-T_0)),\\
J(t) &= B_0 + B\sin(\frac{\pi}{T_0}(t-T_0)).
\end{aligned} \tag{163}$$

This model has period $2T_0$. The parameters are taken as $T_0 = 1,\ A = 4,\ B_0 = 2.3,\ B = 5$.

For the model in Fig. 2E in the main text, the parameters are

When $t \in [0, T_0/2]$,

$$\begin{aligned}
w_1(t) &= A\sin(\frac{\pi}{T_0}t),\\
w_2(t) &= B_0 + B\sin(\frac{\pi}{T_0}t),\\
w_3(t) &= \frac{2A}{T_0}t,\\
J(t) &= B_0 + \frac{2B}{T_0}t,
\end{aligned} \tag{164}$$

when $t \in [T_0/2, T_0]$,

$$\begin{aligned}
w_1(t) &= -\frac{2A}{T_0}(t-T_0),\\
w_2(t) &= B_0 - \frac{2B}{T}(t-T_0),\\
w_3(t) &= A\sin(\frac{\pi}{T_0}t),\\
J(t) &= B_0 + B\sin(\frac{\pi}{T_0}t).
\end{aligned} \tag{165}$$

This model has period $T_0$. The parameters $T_0, A, B_0, B$ take the same values with the former model. The former model is obtained by adding $\pi$ flux on hoppings $w_1$ and $w_3$ at $t = nT_0$ for this model.

The parameters of the model in Fig. 34(b) are

When $t \in [0, T_0/4]$,

$$\begin{aligned}
w_1(t) &= (A + \frac{C-A}{T_0/4}t)\cos(\frac{4\pi}{T_0}t),\\
w_2(t) &= B\cos(\frac{4\pi}{T_0}t),\\
w_3(t) &= (C + \frac{A-C}{T_0/4}t)\cos(\frac{4\pi}{T_0}t),\\
J(t) &= D\cos(\frac{4\pi}{T_0}t),
\end{aligned} \tag{166}$$

when $t \in [T_0/4, T_0]$,

$$\begin{aligned} w_1(t) &= -(C + \frac{A-C}{3T_0/4}(t - \frac{T_0}{4}))|\cos(\frac{4\pi}{3T_0}t + \frac{2\pi}{3})|, \\ w_2(t) &= -B|\cos(\frac{4\pi}{3T_0}t + \frac{2\pi}{3})|, \\ w_3(t) &= -(A + \frac{C-A}{3T_0/4}(t - \frac{T_0}{4}))|\cos(\frac{4\pi}{3T_0}t + \frac{2\pi}{3})|, \\ J(t) &= -D|\cos(\frac{4\pi}{3T_0}t + \frac{2\pi}{3})|, \end{aligned} \tag{167}$$

when $t \in [T_0, 5T_0/4]$,

$$\begin{aligned} w_1(t) &= -(A + \frac{C-A}{T_0/4}(t - T_0))\cos(\frac{4\pi}{T_0}(t - T_0)), \\ w_2(t) &= -B\cos(\frac{4\pi}{T_0}(t - T_0)), \\ w_3(t) &= -(C + \frac{A-C}{T_0/4}(t - T_0))\cos(\frac{4\pi}{T_0}(t - T_0)), \\ J(t) &= -D\cos(\frac{4\pi}{T_0}(t - T_0)), \end{aligned} \tag{168}$$

when $t \in [5T_0/4, 2T_0]$,

$$\begin{aligned} w_1(t) &= (C + \frac{A-C}{3T_0/4}(t - \frac{5T_0}{4}))|\cos(\frac{4\pi}{3T_0}(t - T_0) + \frac{2\pi}{3})|, \\ w_2(t) &= B|\cos(\frac{4\pi}{3T_0}(t - T_0) + \frac{2\pi}{3})|, \\ w_3(t) &= (A + \frac{C-A}{3T_0/4}(t - \frac{5T_0}{4}))|\cos(\frac{4\pi}{3T_0}(t - T_0) + \frac{2\pi}{3})|, \\ J(t) &= D|\cos(\frac{4\pi}{3T_0}(t - T_0) + \frac{2\pi}{3})|. \end{aligned} \tag{169}$$

The period is $2T_0$. The parameters are taken as $T_0 = 1,\ A = -3,\ B = 2,\ C = 5,\ D = 3$. This model has two-fold projective rotation centers at $t = T_0/8 + nT_0$ and ordinary two-fold rotation centers at $t = 5T_0/8 + nT_0$. We can reset $t = t' + T_0/8$, that we have $w_1(-t') = -w_3(t'), w_2(-t') = -w_2(t'), J(-t') = -J(t')$. Now the two-fold rotation centers are at $t' = nT_0$ and $t' = (n + 1/2)T_0$.

The parameters of the model in Fig. 34(a) are

When $t \in [0, T_0/4]$,

$$\begin{aligned} w_1(t) &= (A + \frac{C-A}{T_0/4}t)|\cos(\frac{4\pi}{T_0}t)|, \\ w_2(t) &= B|\cos(\frac{4\pi}{T_0}t)|, \\ w_3(t) &= (C + \frac{A-C}{T_0/4}t)|\cos(\frac{4\pi}{T_0}t)|, \\ J(t) &= D|\cos(\frac{4\pi}{T_0}t)|, \end{aligned} \tag{170}$$

when $t \in [T_0/4, T_0]$,

$$\begin{aligned} w_1(t) &= (C + \frac{A-C}{3T_0/4}(t - \frac{T_0}{4}))|\cos(\frac{4\pi}{3T_0}t + \frac{2\pi}{3})|, \\ w_2(t) &= B|\cos(\frac{4\pi}{3T_0}t + \frac{2\pi}{3})|, \\ w_3(t) &= (A + \frac{C-A}{3T_0/4}(t - \frac{T_0}{4}))|\cos(\frac{4\pi}{3T_0}t + \frac{2\pi}{3})|, \\ J(t) &= D|\cos(\frac{4\pi}{3T_0}t + \frac{2\pi}{3})|. \end{aligned} \tag{171}$$

This model has period $T_0$. The parameters take the same values as the former model. This model has ordinary two-fold rotation centers at $t = T_0/8$ and $t = 5T_0/8$. We also reset $t = t' + T_0/8$. The model in Fig. 34(b) is obtained by adding $\pi$ flux at $t' = 0$ to this model.

### F. References


55. Y. Aharonov and D. Bohm, Phys. Rev. 115, 485 (1959).
56. G. Matteucci and G. Pozzi, Phys. Rev. Lett. 54, 2469 (1985).
57. A. van Oudenaarden, M. H. Devoret, Y. V. Nazarov, and J. E. Mooij, Nature (London) 391, 768 (1998).
58. W. G. van der Wiel, Y. V. Nazarov, S. De Franceschi, T. Fujisawa, J. M. Elzerman, E. W. G. M. Huizeling, S. Tarucha, and L. P. Kouwenhoven, Phys. Rev. B 67, 033307 (2003).
